# Supplementary material for: MAXIM: Multi-Axis MLP for Image Processing
Source: arXiv:2201.02973 source file (2022-04-01)
Supplement: Supplementary file 1 [file MAXIM_CVPR_Supplementary.pdf]

# MAXIM: Multi-Axis MLP for Image Processing (Supplementary Material)

Anonymous CVPR submission

Paper ID 2106

In this manuscript we provide the following material: (1) descriptions of datasets and training details, (2) more details on the proposed architecture, (3) performance vs. complexity, (4) additional experimental results, (5) more visual comparisons, (6) visualization of the learned model weights, and (7) limitations and discussions.

## 1. Datasets and Training Details

All the datasets used in the paper are summarized in Tab. 1. We describe details of training for each dataset in the following. Note that we used the  $\ell_2$  loss for the dehazing task while using the loss defined in the main paper for all the other tasks.

**Image Denoising.** We train our model on 320 high-resolution images provided in SIDD [2] and evaluate on 1,280 ( $256 \times 256$ ) and 1,000 ( $512 \times 512$ ) images provided by authors of SIDD [2] and DND [26], respectively. The results on DND are obtained via the online server [1]. We cropped the training images into  $512 \times 512$  patches with a stride of 256 to prepare the training patches. We trained the MAXIM-3S model for 600k steps with a batch size of 256.

**Image Deblurring.** We train our model on 2,103 image pairs from GoPro [22]. To demonstrate generalization ability, we evaluate our GoPro trained model on 1,111 pairs of GoPro evaluation set, 2,025 images in the HIDE dataset [32], as well as the RealBlur dataset [31] that contains 980 paired images of camera JPEG output and RAW images, respectively. We cropped training images from GoPro into  $512 \times 512$  patches with a stride of 128 to generate training patches. We trained our MAXIM-3S model for 600k steps with a batch size 256. For evaluation on RealBlur setting (2) (see main paper), we loaded GoPro pre-trained checkpoint and fine-tuned with for 70k and 15k iterations on RealBlur-J and RealBlur-R, respectively. Additionally, we trained our model on 24,000 images from the REDS dataset of the NTIRE 2021 Image Deblurring Challenge Track 2 JPEG artifacts [23]. For evaluation, we follow the setting in the NTIRE 2021 Challenge on Image Deblurring [24], i.e. use 300 images in the validation set of REDS.

| Task                            | Dataset             | #Train | #Test | Test Dubname |
|---------------------------------|---------------------|--------|-------|--------------|
| <b>Denoising</b>                | SIDD [2]            | 320    | 40    | SIDD         |
|                                 | DND [26]            | 0      | 50    | DND          |
| <b>Deblurring</b>               | GoPro [22]          | 2103   | 1111  | GoPro        |
|                                 | HIDE [32]           | 0      | 2025  | HIDE         |
|                                 | RealBlur-J [31]     | 3758   | 980   | RealBlur-J   |
|                                 | RealBlur-R [31]     | 3758   | 980   | RealBlur-R   |
|                                 | REDS [23]           | 24000  | 300   | REDS         |
| <b>Deraining</b>                | Rain14000 [11]      | 11200  | 2800  | Test2800     |
|                                 | Rain1800 [39]       | 1800   | 0     | -            |
|                                 | Rain800 [47]        | 700    | 98    | Test100      |
|                                 | Rain100H [39]       | 0      | 100   | Rain100H     |
|                                 | Rain100L [39]       | 0      | 100   | Rain100L     |
|                                 | Rain1200 [46]       | 0      | 1200  | Test1200     |
|                                 | Rain12 [17]         | 12     | 0     | -            |
|                                 | Raindrop [27]       | 861    | 58    | Raindrop-A   |
| <b>Dehazing</b>                 | RESIDE-ITS [15]     | 13990  | 500   | SOTS-Indoor  |
|                                 | RESIDE-OTS [15]     | 313950 | 500   | SOTS-Outdoor |
| <b>Enhancement (Retouching)</b> | MIT-Adobe FiveK [4] | 4500   | 500   | FiveK        |
|                                 | LOL [38]            | 485    | 15    | LOL          |

Table 1. Dataset summary on five image processing tasks.

We trained from scratch for 10k epochs on REDS.

**Image Deraining.** Following [13, 44], we use a composite training set containing 13,712 clean-rain image pairs collected from multiple datasets [11, 17, 39, 39, 46, 47]. Evaluation is performed on five test sets, Rain100H [39], Rain100L [39], Test100 [47], Test1200 [46], and Test2800 [11]. We trained our MAXIM-2S model for 500k steps with a batch size of 512. For the raindrop removal task, we train MAXIM-2S on 861 pairs of training images in Raindrop dataset [27] for 80k steps with a batch size of 512, and evaluate on testset A (58 images) and testset B (239 images), respectively.

**Image Dehazing.** The RESIDE dataset [15] contains two subsets: Indoor Training Set (ITS) which contains 13,990 hazy images generated from 1399 clean ones, and Outdoor Training Set (OTS) that consists of 313,950 hazing images synthesized from 8,970 haze-free outdoor scenes. We evaluate our model on the Synthetic Objective Testing Set (SOTS) [15]: 500 indoor images for ITS-trained, and 500 outdoor images for OTS-trained models, respectively. We

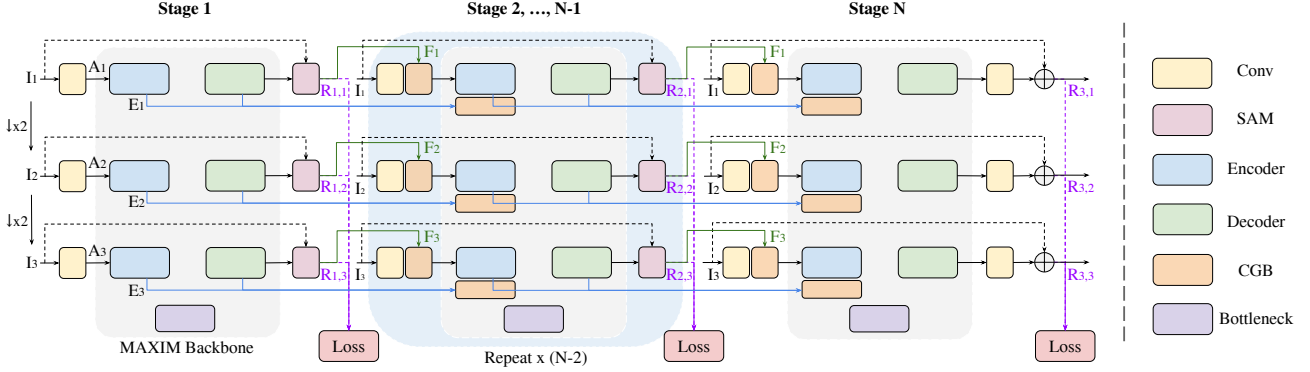

Figure 1. We adopt a general multi-stage framework to improve the performance of MAXIM for challenging restoration tasks. Inspired by [7, 44], we employ the supervised attention module (SAM) and cross-stage feature fusion to help later stages learn. Unlike previous approaches, our MAXIM backbone attains global perception at each layer in each stage due to the proposed multi-axis MLP approaches, making it more powerful in learning global interactions in both low-level and high-level features.

train for 10k and 500 epochs for RESIDE-ITS and RESIDE-OTS using the  $\ell_2$  loss.

**Image Enhancement.** We use the MIT-Adobe FiveK [4] dataset provided by [25] for the retouching evaluation: the first 4,500 images for training and the rest 500 for testing. We cropped training images into  $512 \times 512$  patches with a stride of 256. Moreover, LOL dataset [38] includes 500 pairs of images for low-light enhancement. We train our model on 485 training images and evaluate on 15 test images. We trained for 14k and 180k steps for FiveK and LOL, respectively.

## 2. Architecture Details

Our proposed general multi-stage and multi-scale framework is illustrated in Fig. 1, where each stage uses a single-stage MAXIM backbone, which is illustrated in the main paper. We leverage the multi-scale input-output approach [9] to deeply supervise each stage. Specifically, given an input image  $\mathbf{I} \in \mathbb{R}^{H \times W \times 3}$ , we use the nearest neighbour downscaling method [9] to generate the multi-scale input variants:  $\mathbf{I}_n$ ,  $n = 1, 2, 3$ , while we adopt the bilinear downscaler to produce the ground truth variants:  $\mathbf{T}_n$ ,  $n = 1, 2, 3$ . For each stage, we extract shallow features from the inputs at each scale using  $\text{Conv}3 \times 3$ . Except for the first stage, we fuse the shallow features with attention features coming from the previous supervised attention module (SAM) [44] using a cross gating block (CGB). We also employ cross-stage feature fusion [7, 44] to help later stages, where the intermediate Encoder and Decoder features from the previous stage are fused with features encoded at current stage using a CGB (blue lines in Fig. 1).

### 2.1. Configurations

The detailed specifications of the Encoder part for a single-stage MAXIM are shown in Tab. 2. We also pro-

| Depth | Input shape       | Output Shape      | Layers                                                                                                            |
|-------|-------------------|-------------------|-------------------------------------------------------------------------------------------------------------------|
| 1     | $256^2 \times 3$  | $256^2 \times 32$ | Conv3x3.s1.w32                                                                                                    |
| 1     | $256^2 \times 32$ | $256^2 \times 32$ | CGB* ( $b = d = 16$ )                                                                                             |
| 1     | $256^2 \times 32$ | $256^2 \times 32$ | Conv1x1.s1.w32                                                                                                    |
| 1     | $256^2 \times 32$ | $256^2 \times 32$ | $\left\{ \begin{array}{l} \text{MAB}(b = d = 16) \\ \text{RCAB}(3 \times 3, r = 4) \end{array} \right\} \times 2$ |
| 1     | $256^2 \times 32$ | $128^2 \times 32$ | Conv3x3.s2.w32                                                                                                    |
| 2     | $128^2 \times 32$ | $128^2 \times 64$ | Conv3x3.s1.w64                                                                                                    |
| 2     | $128^2 \times 64$ | $128^2 \times 64$ | CGB* ( $b = d = 16$ )                                                                                             |
| 2     | $128^2 \times 64$ | $128^2 \times 64$ | Conv1x1.s1.w64                                                                                                    |
| 2     | $128^2 \times 64$ | $128^2 \times 64$ | $\left\{ \begin{array}{l} \text{MAB}(b = d = 16) \\ \text{RCAB}(3 \times 3, r = 4) \end{array} \right\} \times 2$ |
| 2     | $128^2 \times 64$ | $64^2 \times 64$  | Conv3x3.s2.w64                                                                                                    |
| 3     | $64^2 \times 64$  | $64^2 \times 128$ | Conv3x3.s1.w128                                                                                                   |
| 3     | $64^2 \times 128$ | $64^2 \times 128$ | CGB* ( $b = d = 8$ )                                                                                              |
| 3     | $64^2 \times 128$ | $64^2 \times 128$ | Conv1x1.s1.w128                                                                                                   |
| 3     | $64^2 \times 128$ | $64^2 \times 128$ | $\left\{ \begin{array}{l} \text{MAB}(b = d = 8) \\ \text{RCAB}(3 \times 3, r = 4) \end{array} \right\} \times 2$  |
| 3     | $64^2 \times 128$ | $32^2 \times 128$ | Conv3x3.s2.w128                                                                                                   |
| 4     | $32^2 \times 128$ | $32^2 \times 256$ | Conv1x1.s1.w256                                                                                                   |
| 4     | $32^2 \times 256$ | $32^2 \times 256$ | $\left\{ \begin{array}{l} \text{MAB}(b = d = 8) \\ \text{RCAB}(1 \times 1, r = 4) \end{array} \right\} \times 2$  |
| 4     | $32^2 \times 256$ | $32^2 \times 256$ | Conv1x1.s1.w256                                                                                                   |
| 4     | $32^2 \times 256$ | $32^2 \times 256$ | $\left\{ \begin{array}{l} \text{MAB}(b = d = 16) \\ \text{RCAB}(1 \times 1, r = 4) \end{array} \right\} \times 2$ |

Table 2. Detailed architectural specifications of the Encoder part of a single-stage MAXIM backbone. Depth 1-3 denotes Encoder blocks, while depth 4 corresponds to Backbone blocks. Note that in Bottlenecks, we use  $\text{Conv}1 \times 1$  in RCAB. \* indicates layers that are not employed in the first stage.

vide input and output shapes of each block and layer. Here  $\text{Conv}3 \times 3_{s1.w32}$  means a Conv layer with  $3 \times 3$  kernels, stride 1, and 32 channels. MAB and RCAB are the two major components in Encoder / Decoder / Bottleneck. Note that in Bottleneck blocks, we use  $(\text{Conv}1 \times 1)$  layers to replace  $\text{Conv}3 \times 3$  in RCAB.

The Decoder part of MAXIM is symmetric with respect to Tab. 2, and has the same configuration. For the CGB

| Model           | Complexity         | Fully-conv | Global |
|-----------------|--------------------|------------|--------|
| MLP-Mixer [35]  | $\mathcal{O}(N^2)$ | ✗          | ✓      |
| gMLP [18]       | $\mathcal{O}(N^2)$ | ✗          | ✓      |
| Swin-Mixer [21] | $\mathcal{O}(N)$   | ✓          | ✗      |
| MAXIM (ours)    | $\mathcal{O}(N)$   | ✓          | ✓      |

Table 3. Comparisons of MAXIM with other MLP models. Our model is both fully-convolutional and global, having a linear complexity with respect to the number of pixels  $N$ .

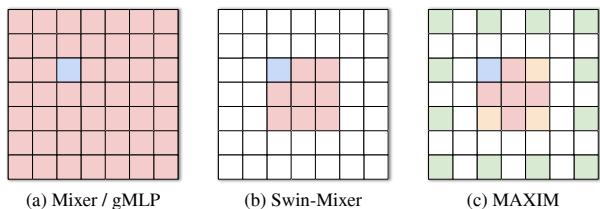

Figure 2. Visualizations of effective receptive fields (shaded area) of the blue pixel for (a) Mixer/gMLP, (b) Swin-Mixer, and (c) our MAXIM. MAXIM attains both local (red) and (dilated) global (green) perception. Yellow pixels are achievable by both local and global branches.

necks, we used  $b = d = 16$  for the depths 1 and 2 while  $b = d = 8$  is adopted for depth 3. Basically, we set the block and grid sizes as 16 for high-resolution stages (*i.e.* feature size  $\geq 128$ ) and 8 for low-resolution stages (*i.e.* feature size  $< 128$ ). Consequently, the input images need to have both dimensions to be divisible by 64, requiring the images to be padded by a multiplier of 64 during the inference.

## 2.2. Comparison with Other MLPs

In Fig. 2, we show a visual comparison of the approximated effective receptive fields among recent MLP models: MLP-Mixer [35], gMLP [18], Swin-Mixer [21], and our proposed MAXIM. Our approach achieves sparse interactions to obtain both local (red in Fig. 2c) and global dilated (green) spatial communications. Moreover, as shown in Tab. 3, unlike previous MLP models, MAXIM obtains both global and fully-convolutional properties with a linear complexity with respect to the number of pixels  $N$ .

## 2.3. JAX Implementations

Here we provide a JAX [3] implementation of the key component of MAXIM, namely the multi-axis gated MLP block (MAB), in Algorithm 1.

## 3. Performance vs. Complexity

We demonstrate the performance vs. complexity trade-off in Tab. 4 as compared with other competing methods for all the tasks. As it can be seen, our model obtains the state-of-the-art performance at a very moderate complexity. On

| Task    | Dataset           | Model           | PSNR  | Params | FLOPs |
|---------|-------------------|-----------------|-------|--------|-------|
| Denoise | SIDD [2]          | MPRNet [44]     | 39.71 | 15.7M  | 1176G |
|         |                   | MIRNet [43]     | 39.72 | 31.7M  | 1572G |
|         |                   | <b>MAXIM-3S</b> | 39.96 | 22.2M  | 339G  |
| Deblur  | GoPro [22]        | MPRNet [44]     | 32.66 | 20.1M  | 1554G |
|         |                   | HINet [7]       | 32.71 | 88.7M  | 341G  |
|         |                   | IPT [6]         | 32.58 | 114M   | 1188G |
|         |                   | <b>MAXIM-3S</b> | 32.86 | 22.2M  | 339G  |
| Derain  | Rain13k (Average) | MSPFN [13]      | 30.75 | 21.7M  | -     |
|         |                   | MPRNet [44]     | 32.73 | 3.64M  | 297G  |
|         |                   | <b>MAXIM-2S</b> | 33.24 | 14.1M  | 216G  |
| Dehaze  | Indoor [15]       | MSBDN [10]      | 33.79 | 31.3M  | 83G   |
|         |                   | FFA-Net [28]    | 36.36 | 4.5M   | 576G  |
|         |                   | <b>MAXIM-2S</b> | 39.72 | 14.1M  | 216G  |
| Enhance | LOL [38]          | MIRNet [43]     | 24.14 | 31.7M  | 1572G |
|         |                   | <b>MAXIM-2S</b> | 23.43 | 14.1M  | 216G  |

Table 4. Model performance vs. complexity comparison of our model with other competing methods for all the tasks. FLOPs are calculated on an input image of size  $256 \times 256$ .

| Method          | REDS [23]    |              |
|-----------------|--------------|--------------|
|                 | PSNR         | SSIM         |
| MPRNet [44]     | 28.79        | 0.911        |
| HINet [7]       | <u>28.83</u> | <u>0.862</u> |
| <b>MAXIM-3S</b> | <b>28.93</b> | <b>0.865</b> |

Table 5. Deblurring comparisons on REDS. Our method outperforms previous winning solution (HINet) on the REDS dataset of NTIRE 2021 Image Deblurring Challenge Track 2 JPEG artifacts. The scores are evaluated on 300 images from the validation set. Results are gathered from the authors of [7].

| Method          | Raindrop-A [27] |              | Raindrop-B [27] |              |
|-----------------|-----------------|--------------|-----------------|--------------|
|                 | PSNR            | SSIM         | PSNR            | SSIM         |
| AGAN [27]       | <u>31.62</u>    | 0.921        | 25.05           | 0.811        |
| DuRN [20]       | 31.24           | 0.926        | <u>25.32</u>    | <u>0.817</u> |
| Quan [29]       | 31.36           | <u>0.928</u> | -               | -            |
| <b>MAXIM-2S</b> | <b>31.87</b>    | <b>0.935</b> | <b>25.74</b>    | <b>0.827</b> |

Table 6. Deraining comparisons on Raindrop removal dataset [27]. Our MAXIM-2S model attains state-of-the-art performance on both Raindrop testset A and B.

denoising, for example, MAXIM-3S has only 21% FLOPs and 70% parameters of MIRNet [43]; on deblurring, our MAXIM-3S model requires only 25% of the number of parameters of the previous best model HINet [7], and merely 19% of the number of parameters in the Transformer-based model IPT [6]. It is also worth noting that unlike IPT, our model requires no large-scale pre-training to obtain leading performance, making it attractive for low-level tasks where datasets are often at limited scale.

## 4. Additional Experiments

Due to limited space in the main paper, we also show experimental results on deblurring and raindrop removal.

**Deblurring on REDS [23].** Tab. 5 shows the quantitative comparison of MAXIM-3S against the winning solution, HINet [7], and a leading model, MPRNet [44] on the REDS dataset of NTIRE 2021 Image Deblurring Challenge Track 2 JPEG artifacts [23]. The metrics are computed and averaged on 300 validation images. Our MAXIM-3S model surpasses HINet by **0.1** dB of PSNR.

**Raindrop removal [27].** Apart from the rain streak removal task reported in the main paper, we also evaluated our MAXIM model on the raindrop removal task. As can be seen in Tab. 6, our model achieves the best performance: **31.87** dB and **25.74** dB PSNR on Raindrop testset A and B.

## 5. More Visual Comparisons

**Denoising.** Fig. 4 shows denoising results of our model compared with SOTA models on SIDD [2]. Our model recovers more details, yielding visually pleasant outputs.

**Deblurring.** The visual results on GoPro [22], HIDE [32], RealBlur-J [31], and REDS [23] are shown in Fig. 5, Fig. 6, Fig. 7, and Fig. 8, respectively. Our model outperforms other competing methods on both synthetic and real-world deblurring benchmarks.

**Deraining.** The qualitative comparisons of our model against SOTA on deraining are shown in Fig. 9, Fig. 10, Fig. 11, and Fig. 12.

**Raindrop removal.** We provide the visual comparisons for the raindrop removal task on the Raindrop testset A and B [27] in Fig. 13 and Fig. 14.

**Dehazing.** We provide dehazing comparisons on the SOTS [15] indoor and outdoor sets in Fig. 15 and Fig. 16.

**Retouching.** Fig. 17 shows additional comparisons of our model with competing methods on the Five-K dataset [4] provided by [25] for retouching results.

**Low-light enhancement.** Fig. 18 demonstrates the evaluations on the LOL [38] test set for low-light enhancement.

## 6. Weight Visualizations

Fig. 3 visualizes the spatial projection matrices of the block gMLP and the grid gMLP layers in each stage of MAXIM-3S trained for GoPro [22] deblurring. Similar to [18], we also observed that the weights after learning exhibit locality and spatial invariance. Surprisingly, the global grid gMLP layer also learns to perform ‘local’ operations (but on the uniform dilated grid). The spatial weights of block gMLP and grid gMLP in the same layer often demonstrate similar or coupled shapes, which may be attributed to the parallel-branch design in the multi-axis gMLP block. However, we have not observed a clear trend on how these filters at different stages vary.

## 7. Limitations and Discussions

One potential limitation of our model, which is shared with the existing SOTA, is the relatively inadequate generalization to real-world examples. This perhaps can be attributed to the training examples provided by the existing synthesized image restoration benchmarks. Creating more realistic, large-scale datasets through data-generation schemes [33, 37] can improve this shortcoming. Also, we observed that our model tends to slightly overfit certain benchmarks, because we did not apply a strong regularization (*e.g.*, dropout) during training. Even though we find that regularization may result in a small reduction in the performance, it is worth exploring in future to effectively improve the generalization of our restoration models.

It is worth mentioning that our model is able to generate high quality sharp images, which are visually comparable to the state-of-the-art generative models [14, 49]. However, our model produces more conservative results without hallucinating many nonexistent details, delivering more reliability against generative models.



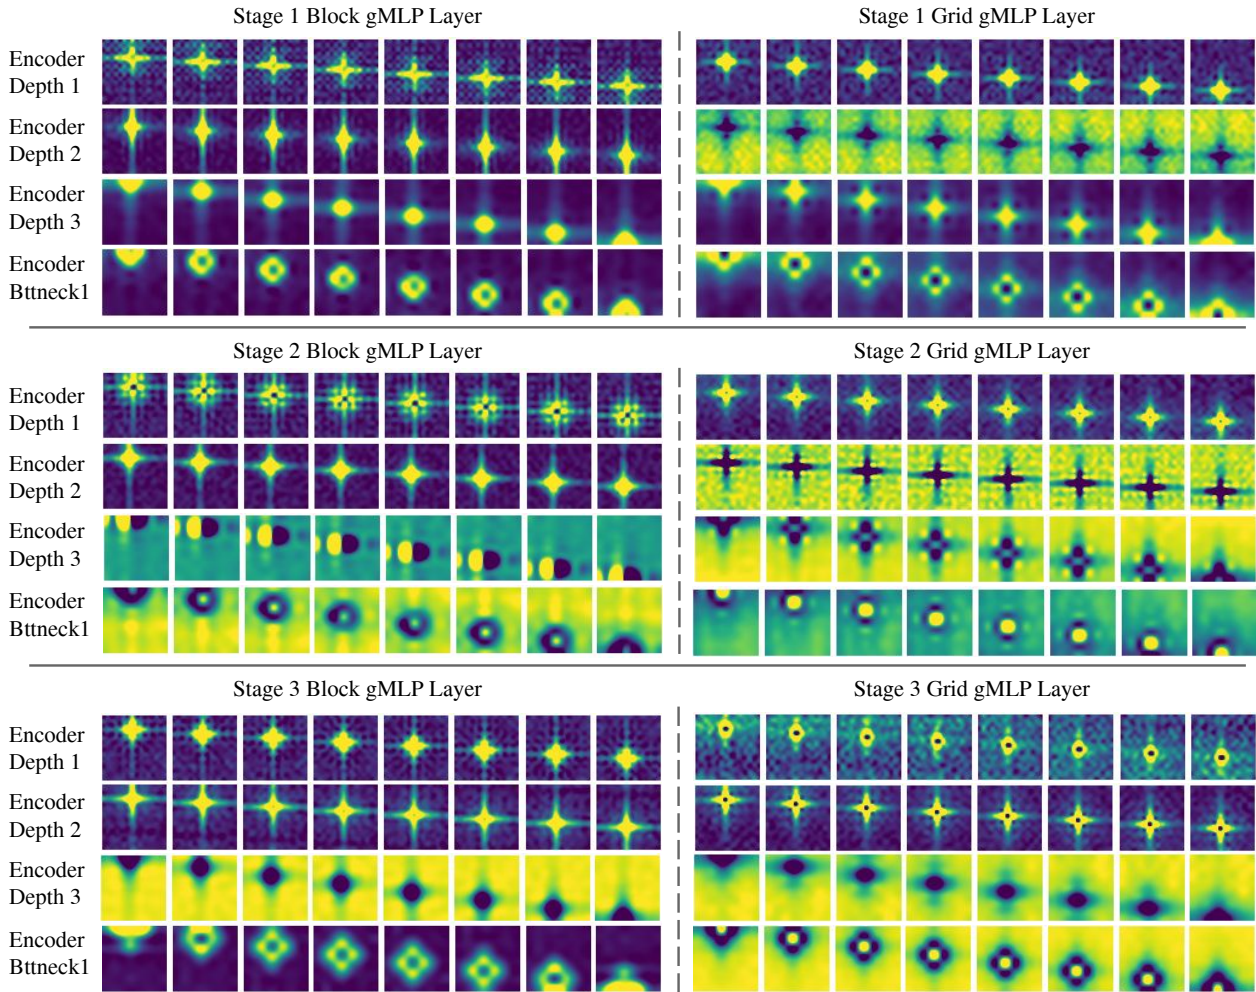

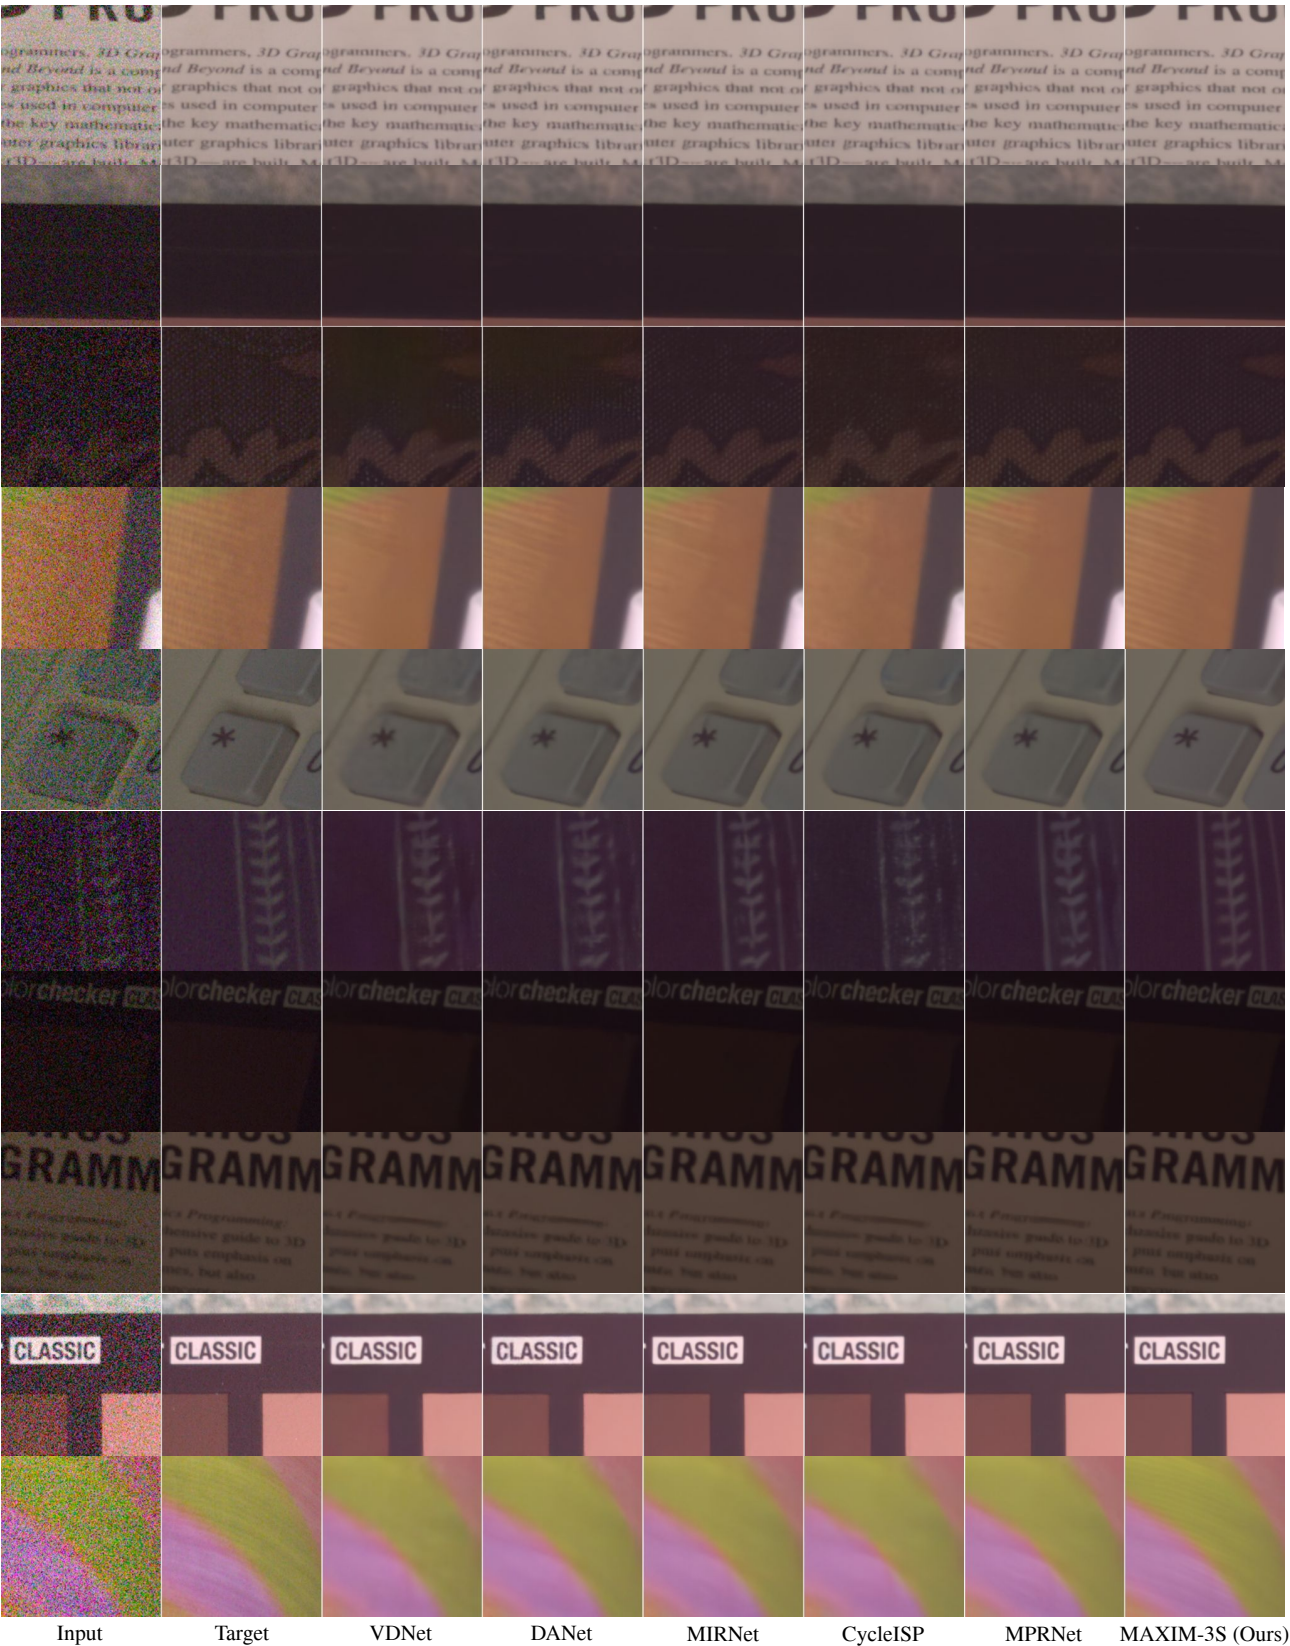

Input Target VNet DANet MIRNet CycleISP MPRNet MAXIM-3S (Ours)

Figure 4. Visual examples for image denoising on SIDD [2] among VDN [40], DANet [41], MIRNet [43], CycleISP [42], MPRNet [44], and our proposed MAXIM-3S model.



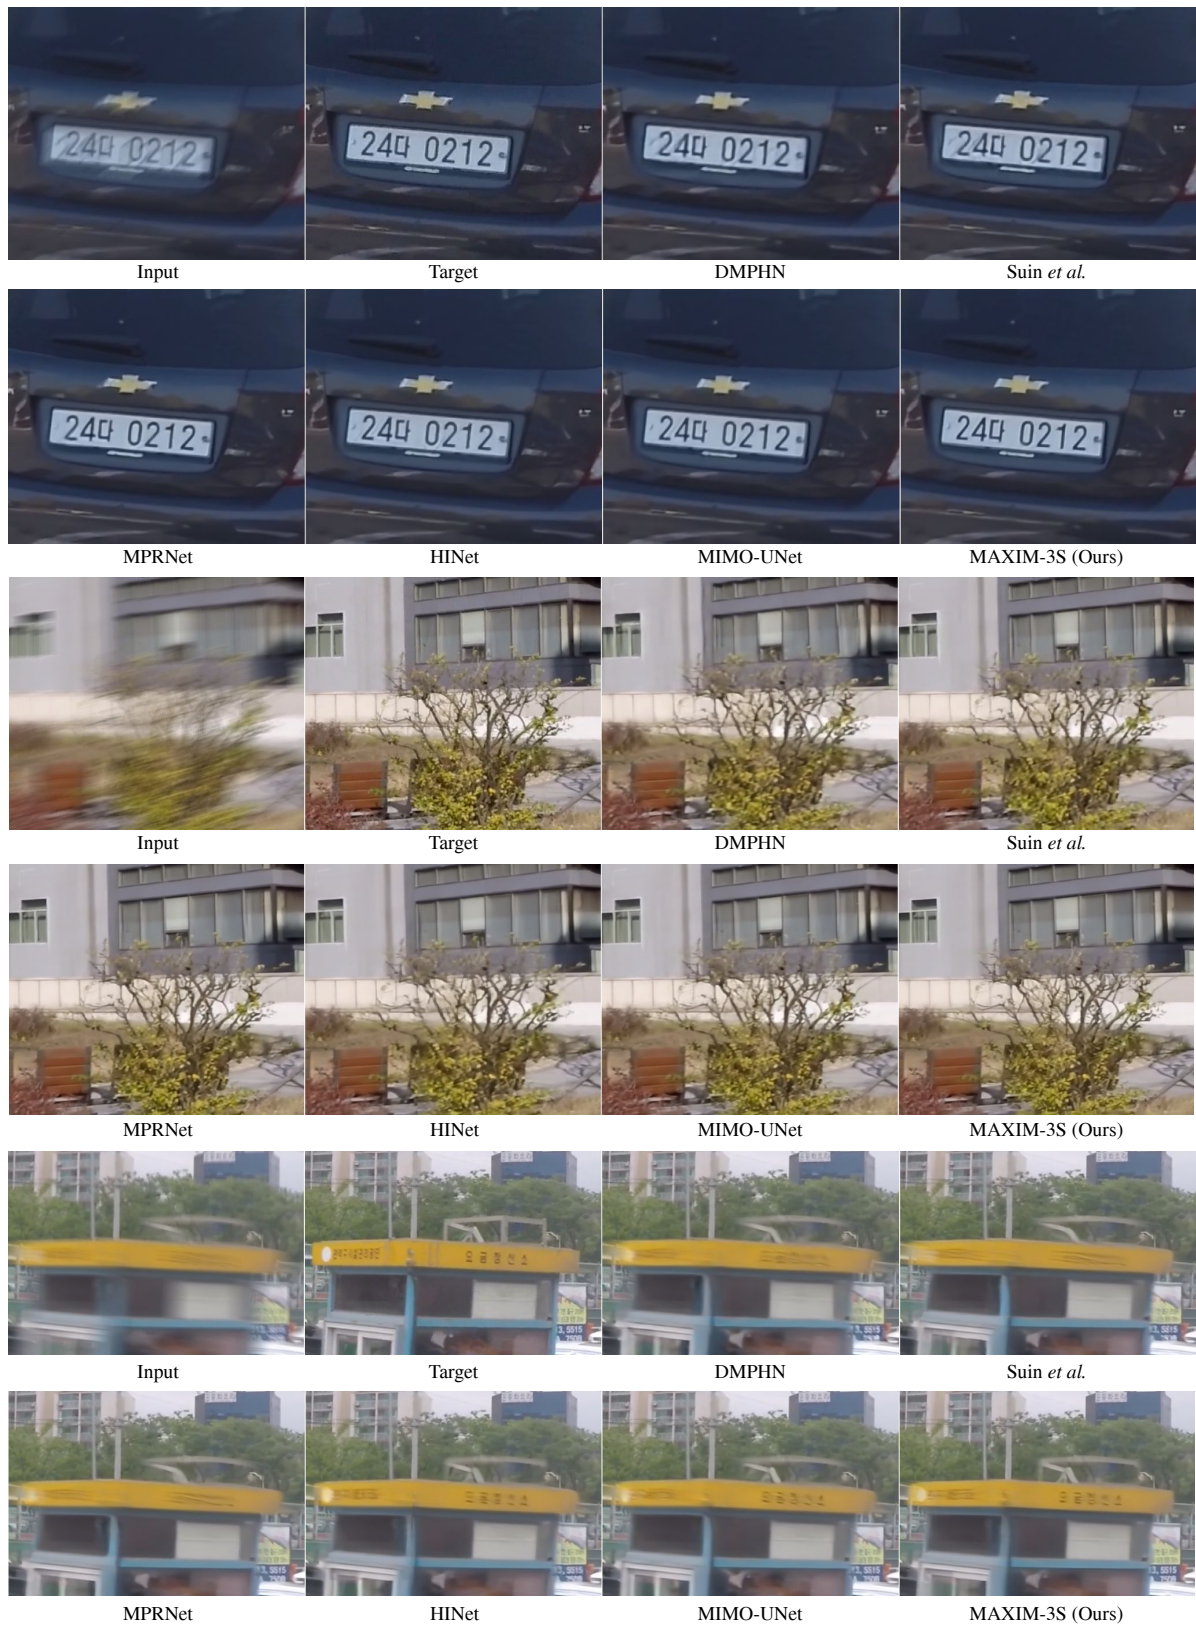

Figure 5. Visual examples for image deblurring on GoPro [22] among DMPHN [45], Suin et al. [34], MPRNet [44], HINet [7], MIMO-UNet [9], and our MAXIM-3S.



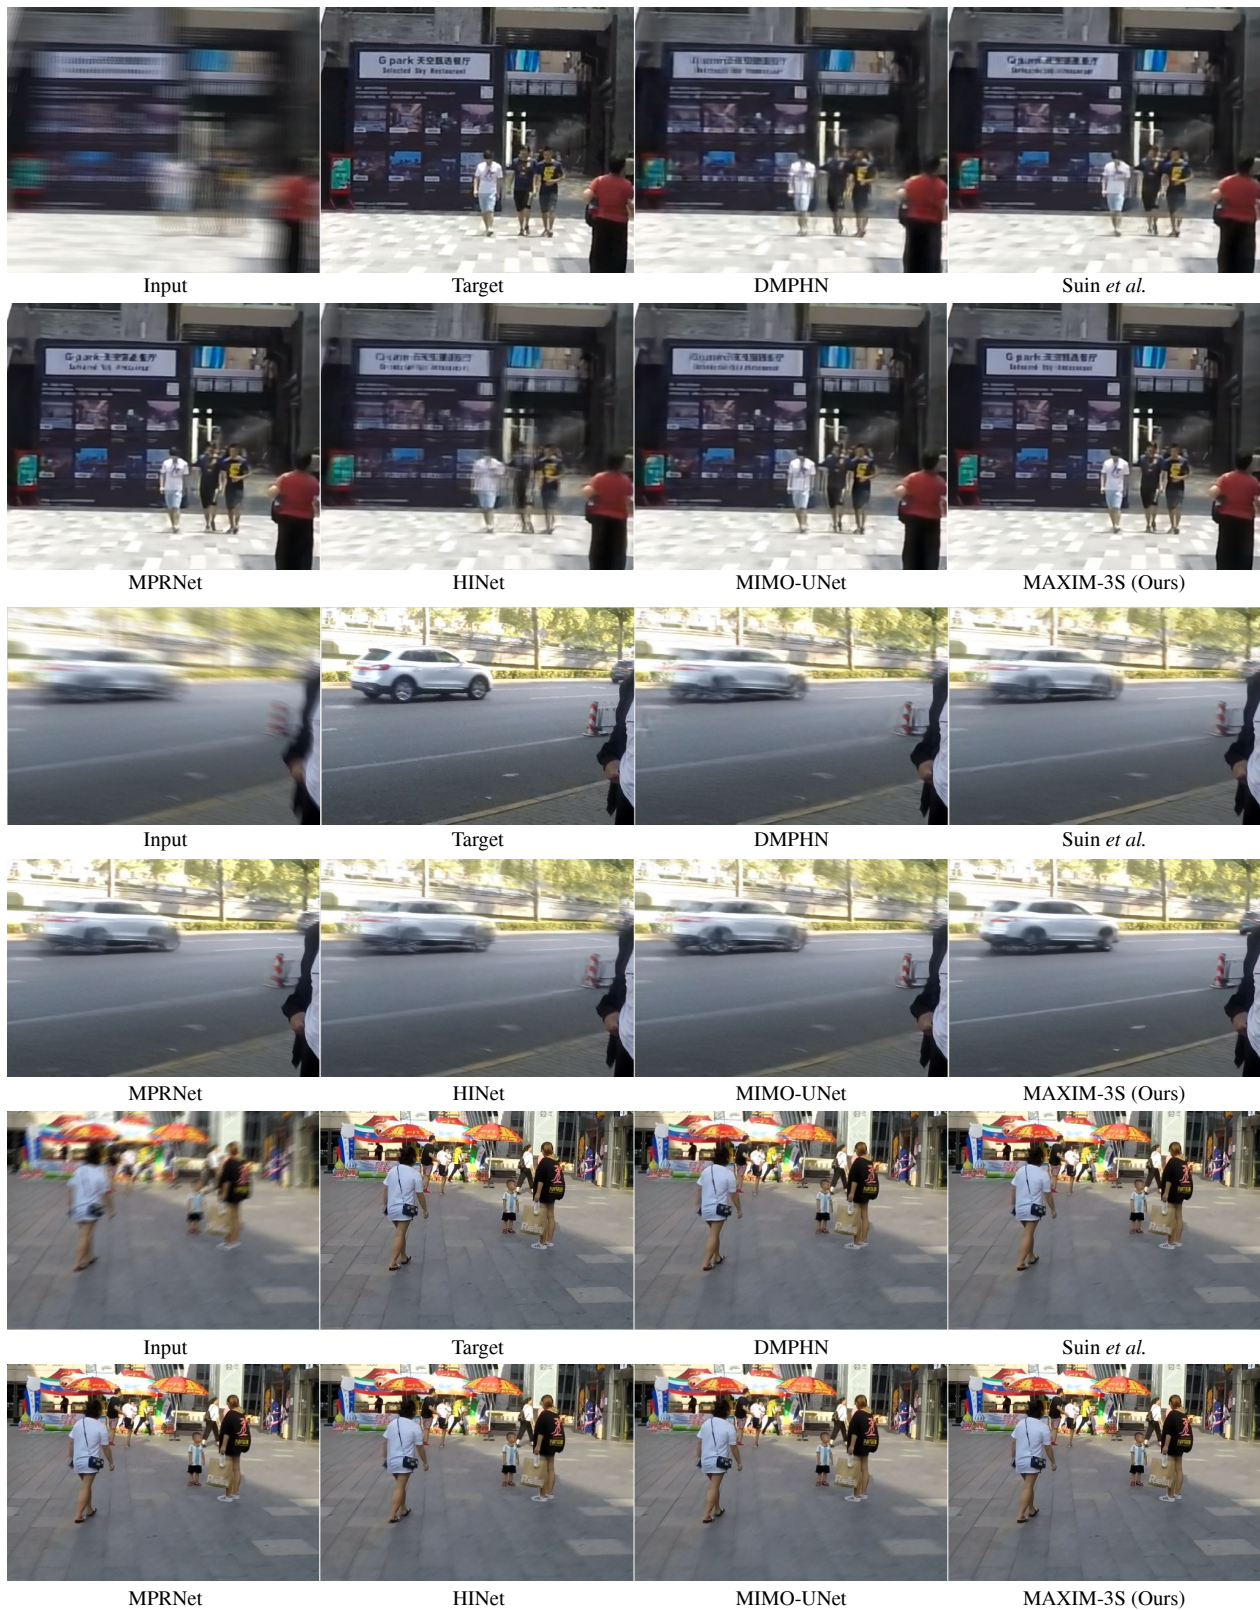

Figure 6. Visual comparisons for image deblurring on HIDE [32] among DMPHN [45], Suin *et al.* [34], MPRNet [44], HINet [7], MIMO-UNet [9], and our MAXIM-3S.



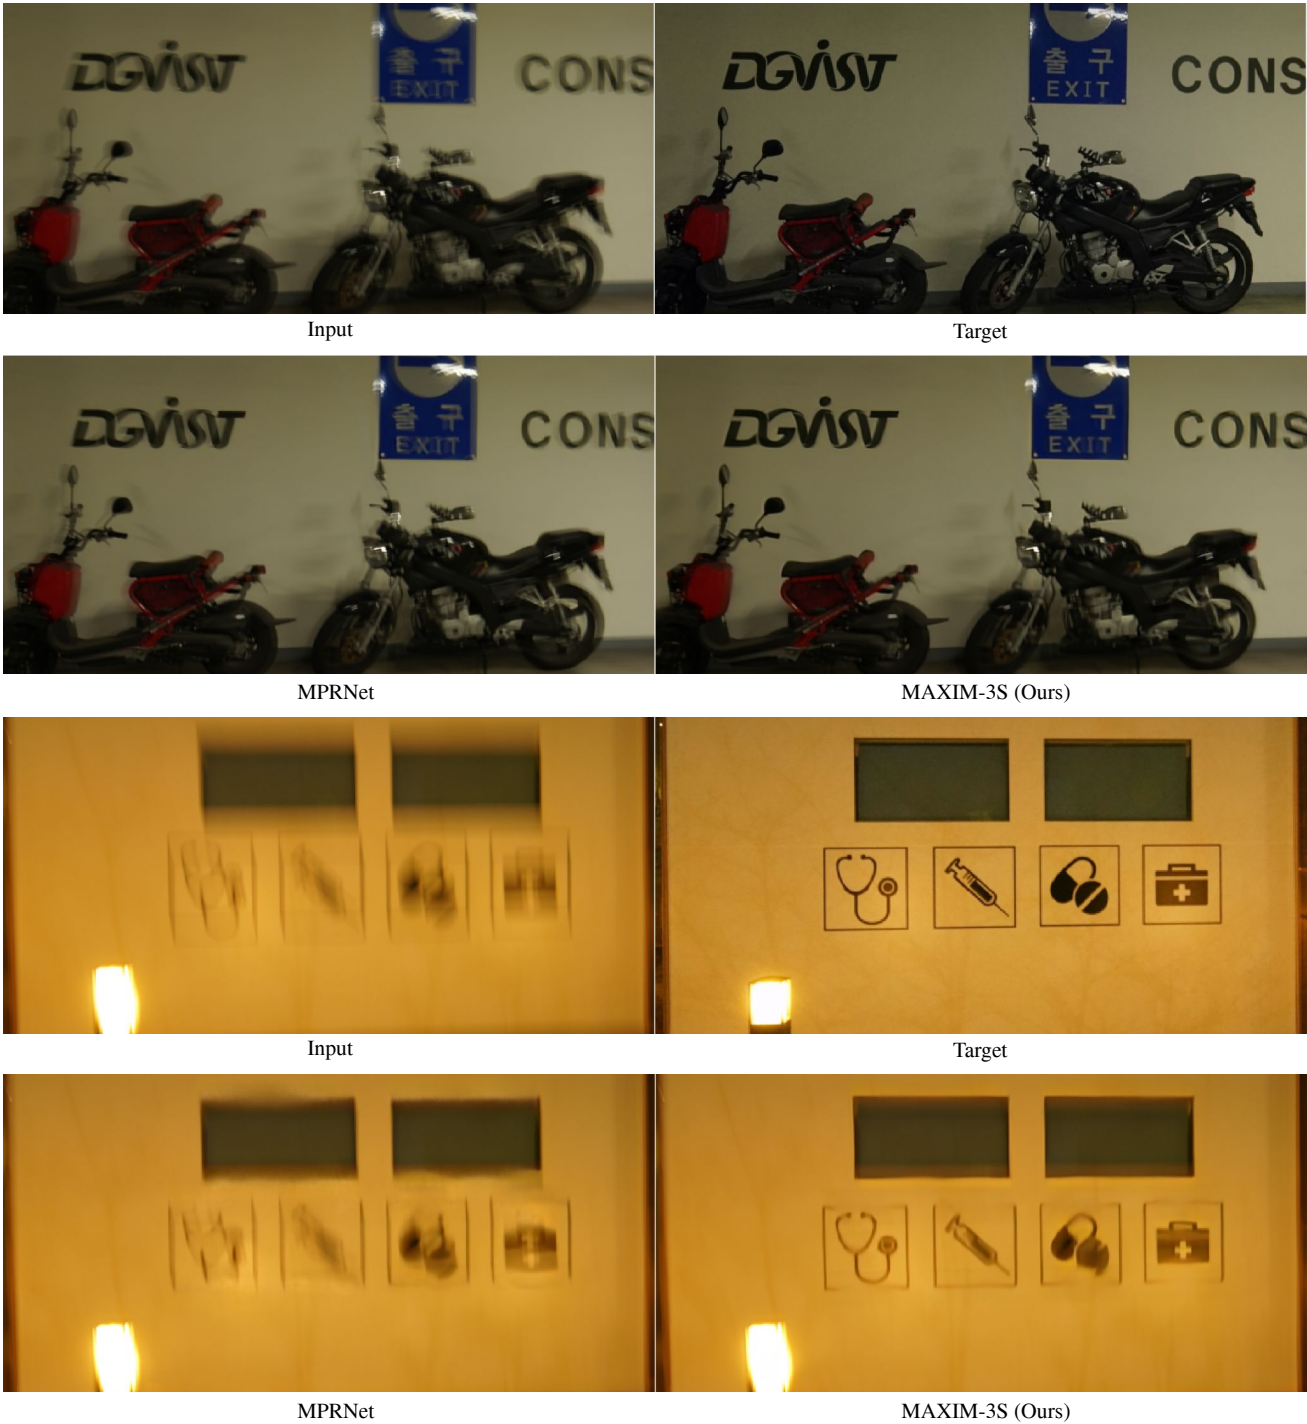

Figure 7. Visual comparisons for image deblurring on RealBlur-J [31] between previous best model MPRNet [44] and MAXIM-3S.

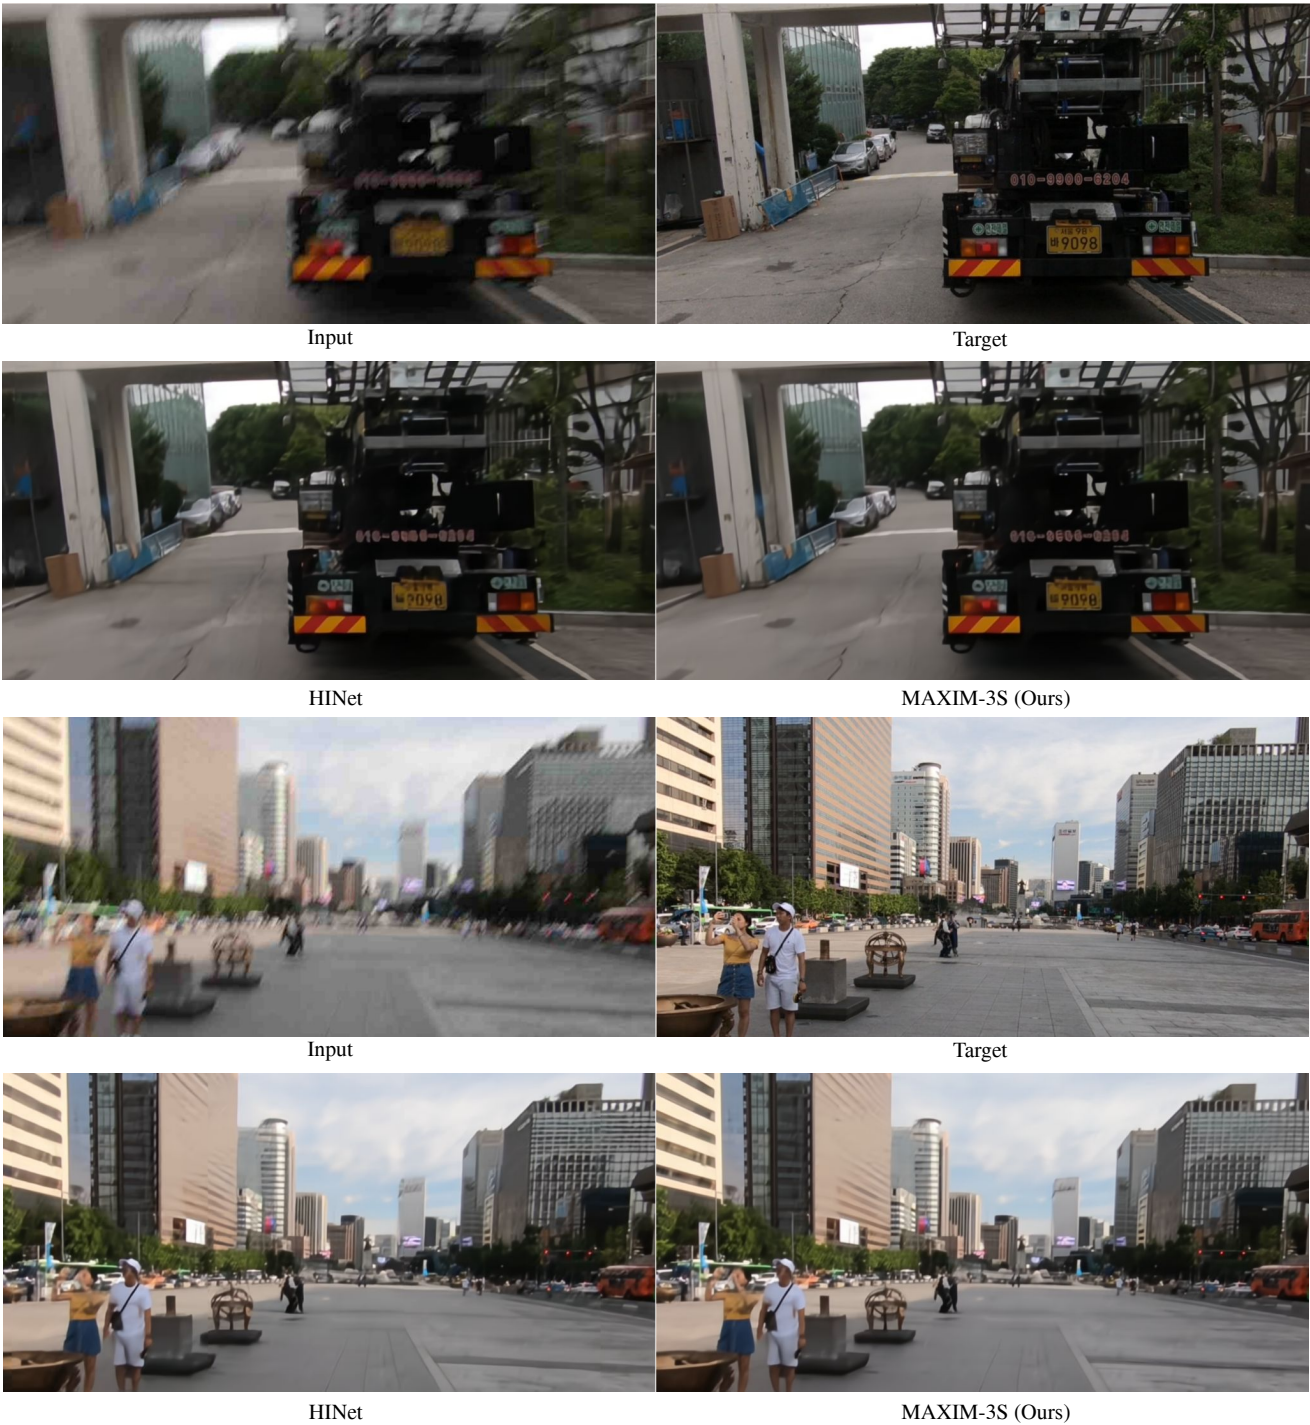

Figure 8. Visual comparisons for image deblurring on REDS [23] between our model and the winning solution for REDS dataset of the NTIRE 2021 Image Deblurring Challenge Track 2 JPEG artifacts [23].



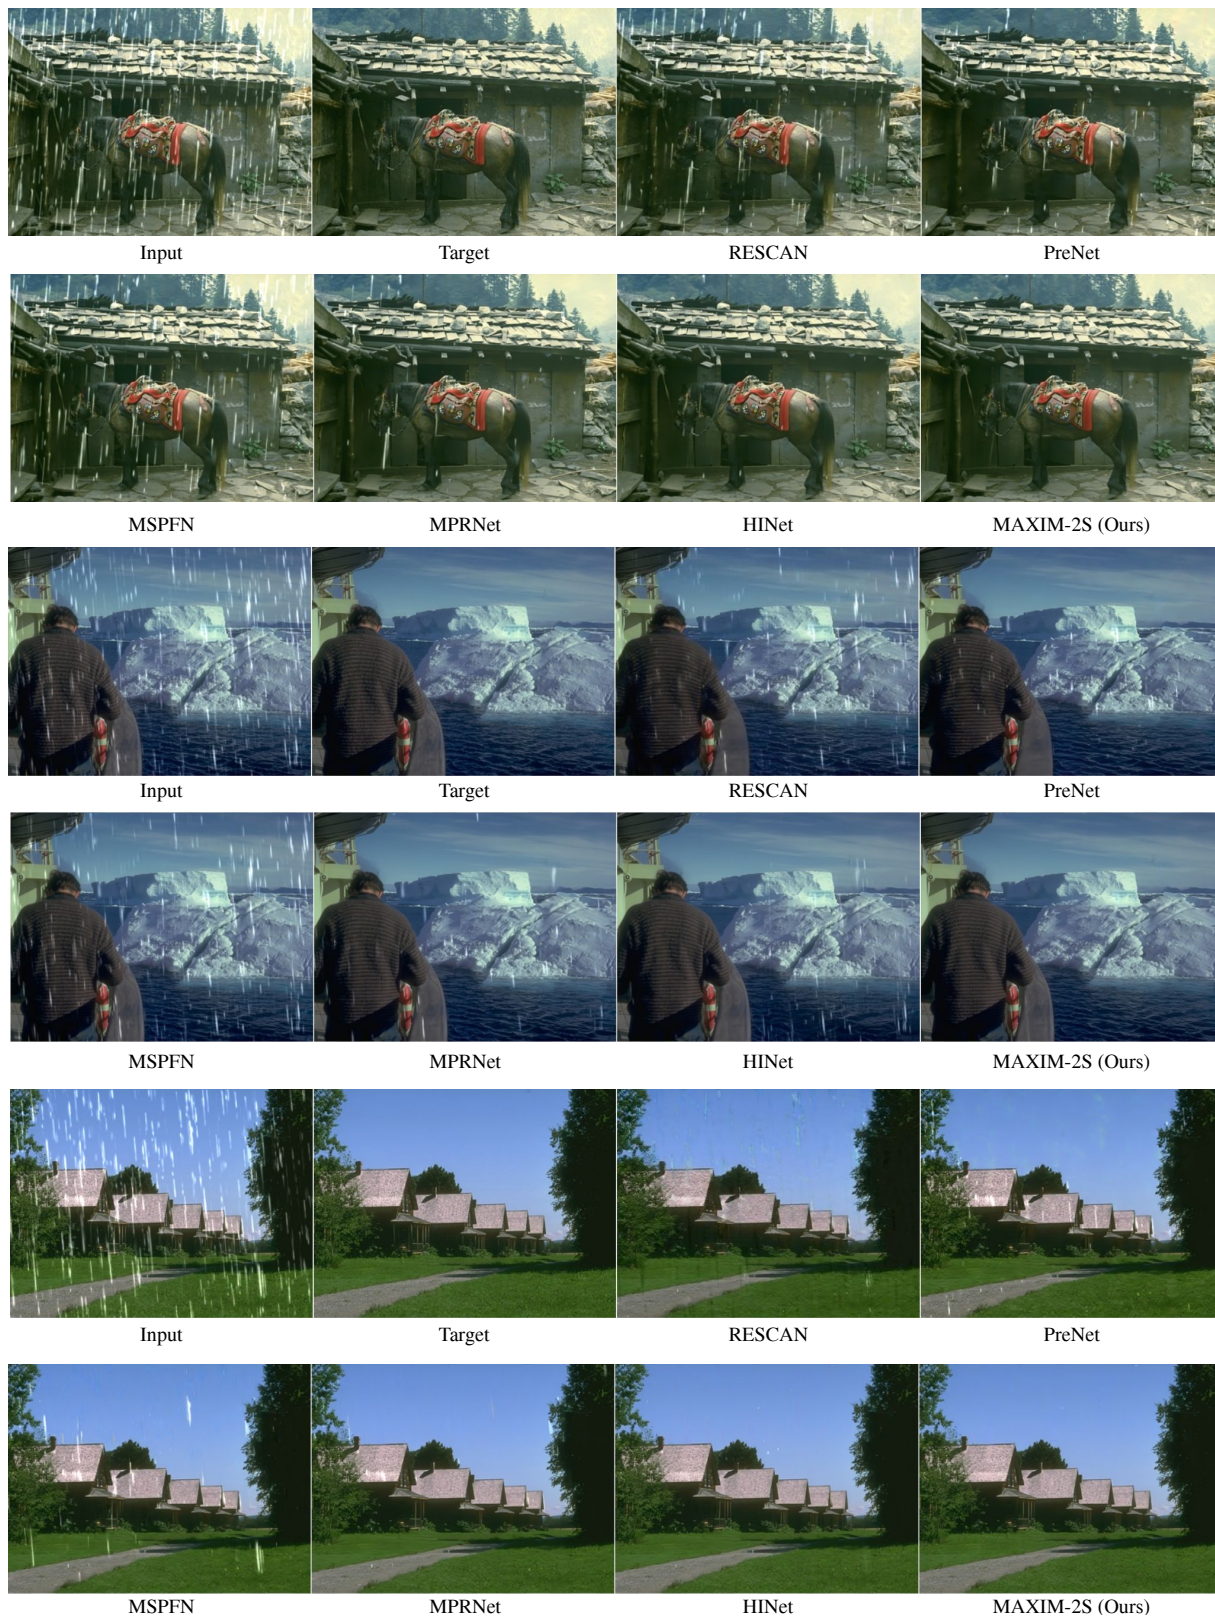

Figure 9. Visual examples for image deraining on Rain100L [39] among RESCAN [16], PreNet [30], MSPFN [13], MPRNet [44], HINet [7], and our MAXIM-2S model.



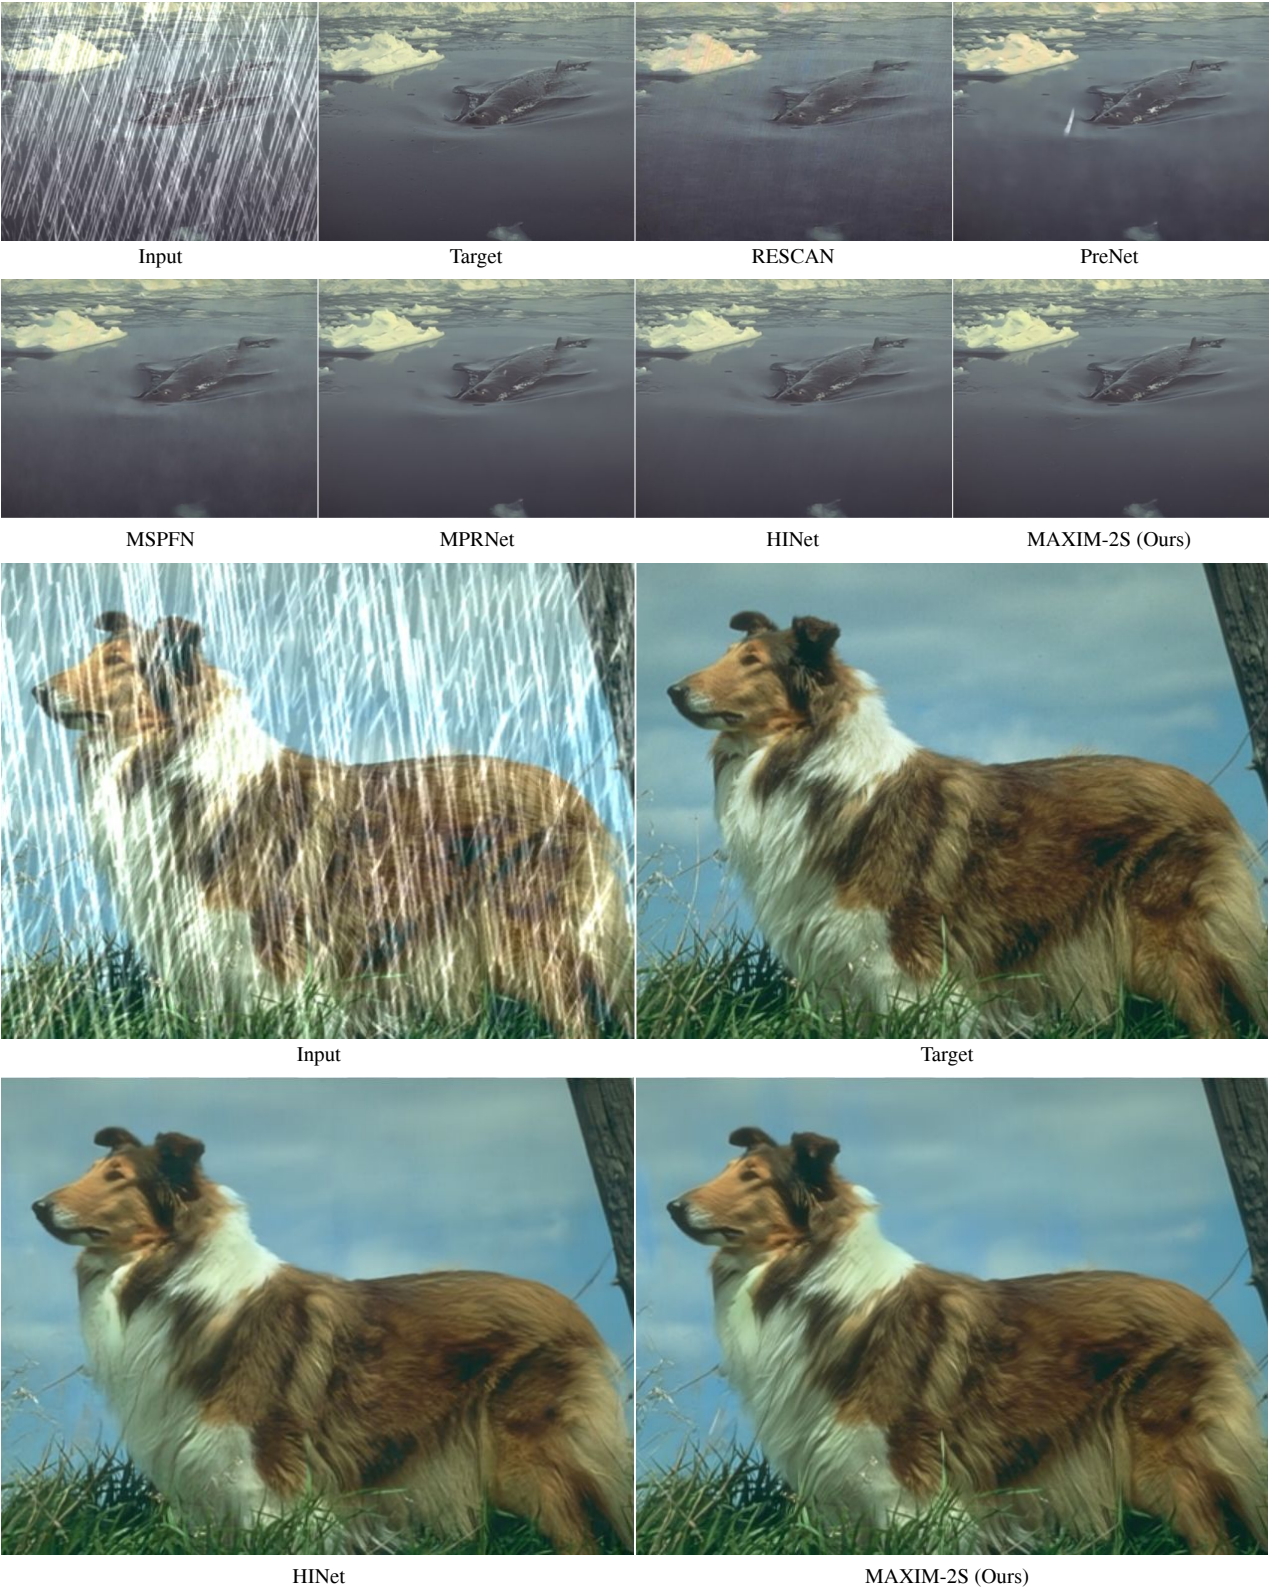

Figure 10. Visual examples for image deraining on Rain100H [39]. At extremely high raining levels, our model recovers more details and textures compared to previous competitive methods.



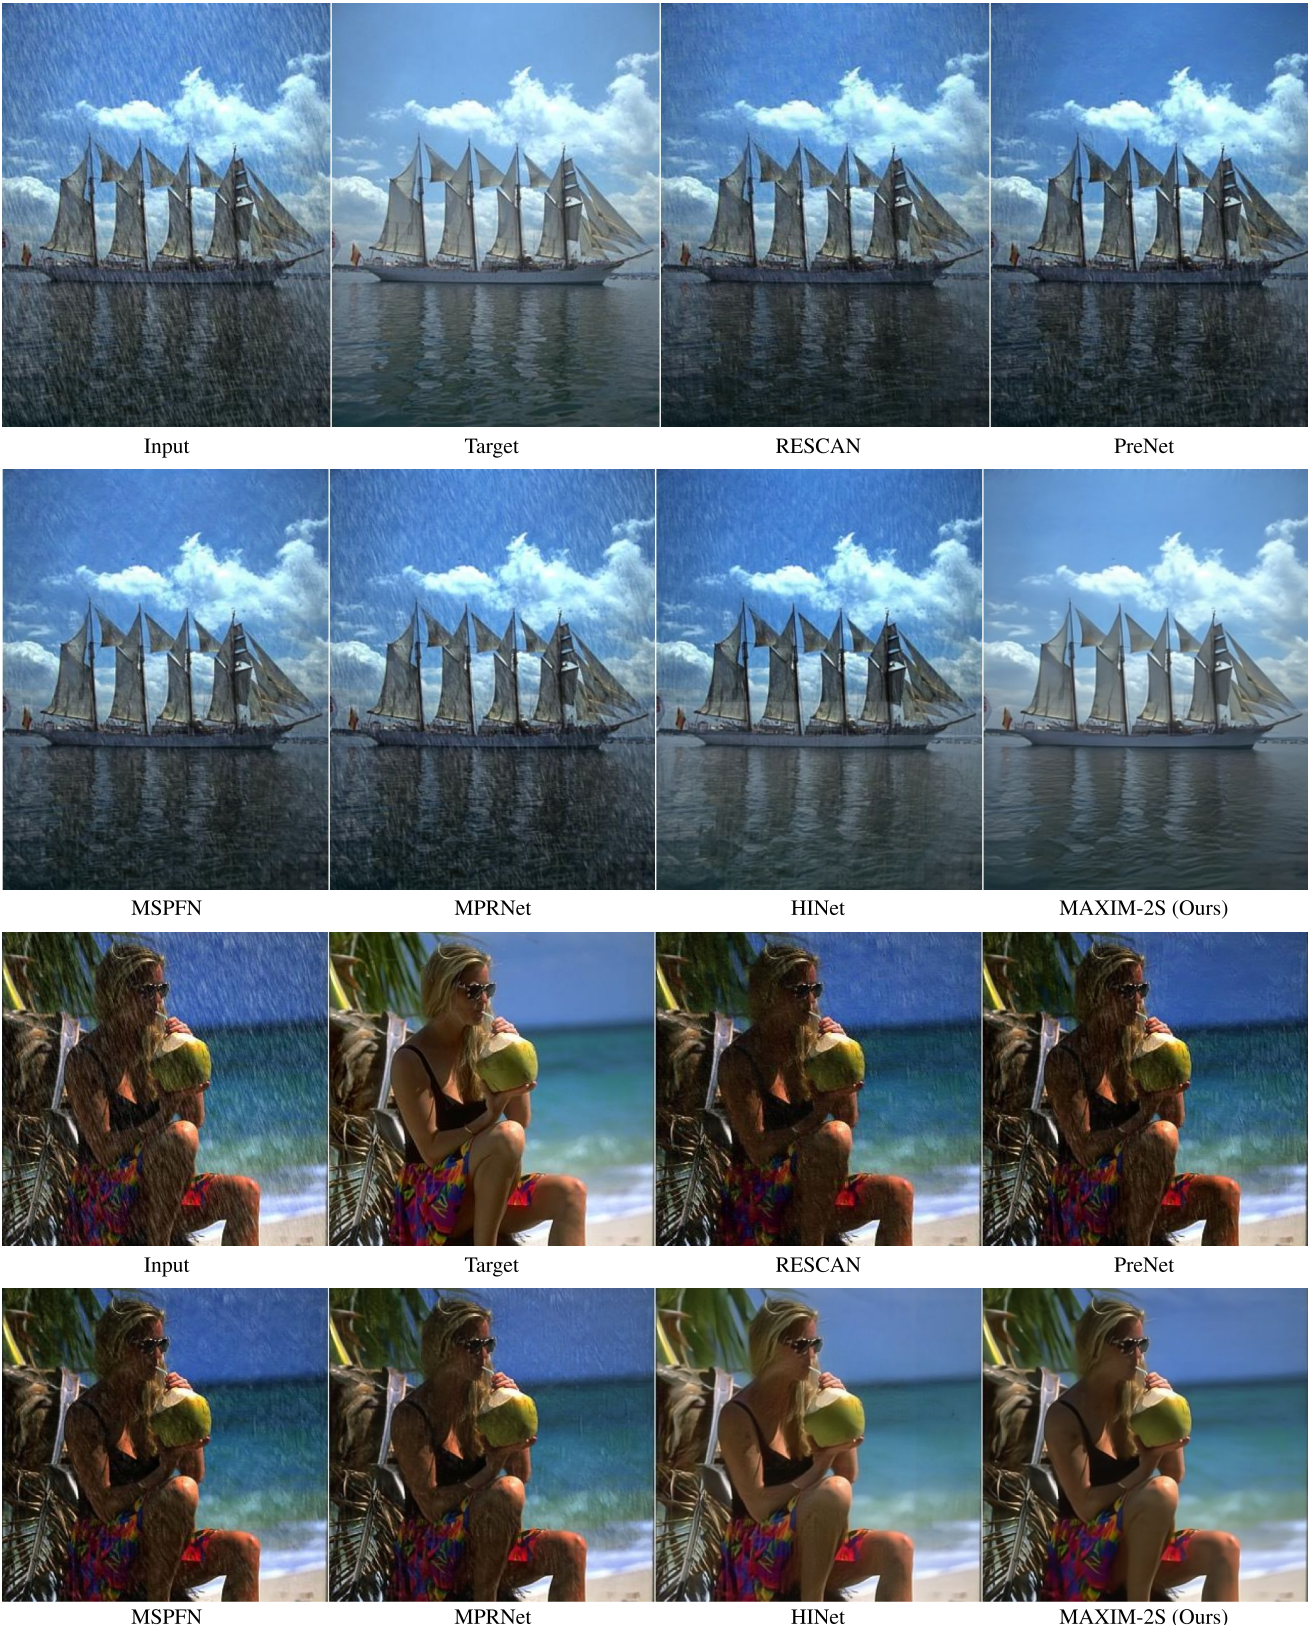

Figure 11. Visual examples for image deraining on Test100 [47]. Our model removes both raining streaks and visible JPEG artifacts.



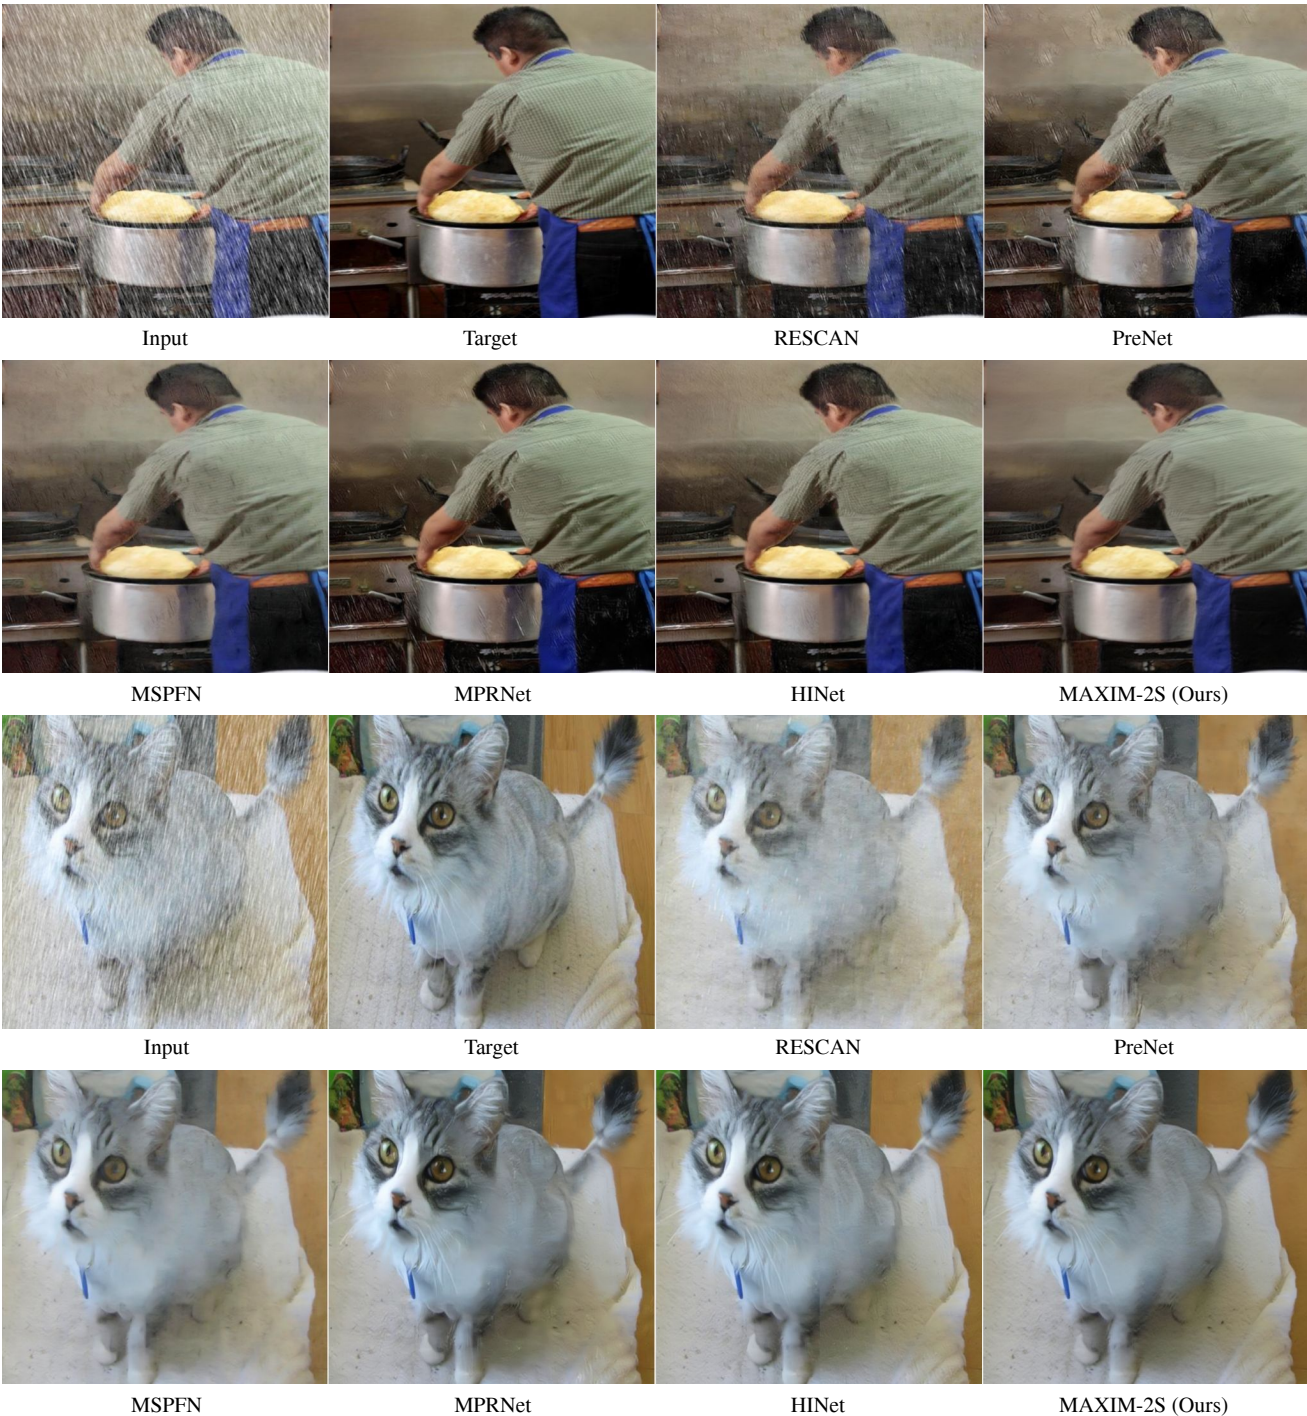

Figure 12. Visual examples for image deraining on Test1200 [46].



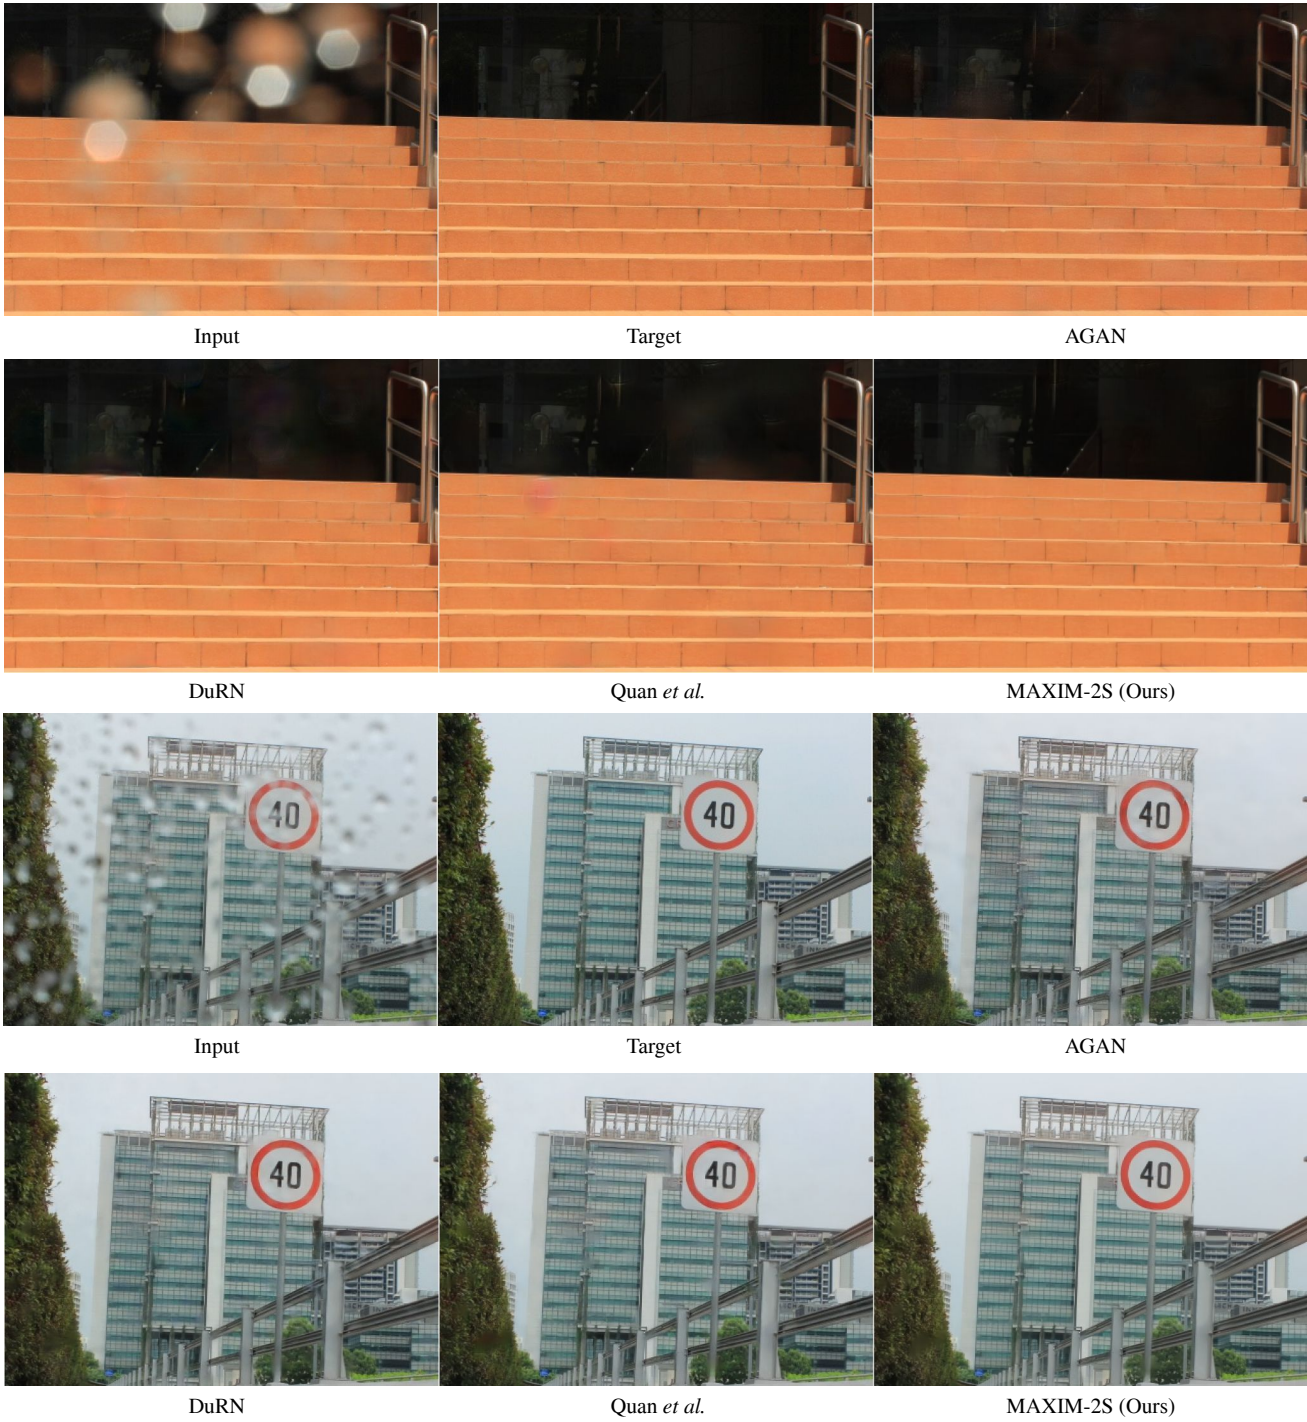

Figure 13. Visual comparisons for raindrop removal on Raindrop-A [27] among AGAN [27], DuRN [20], Quan [29], and MAXIM-2S.



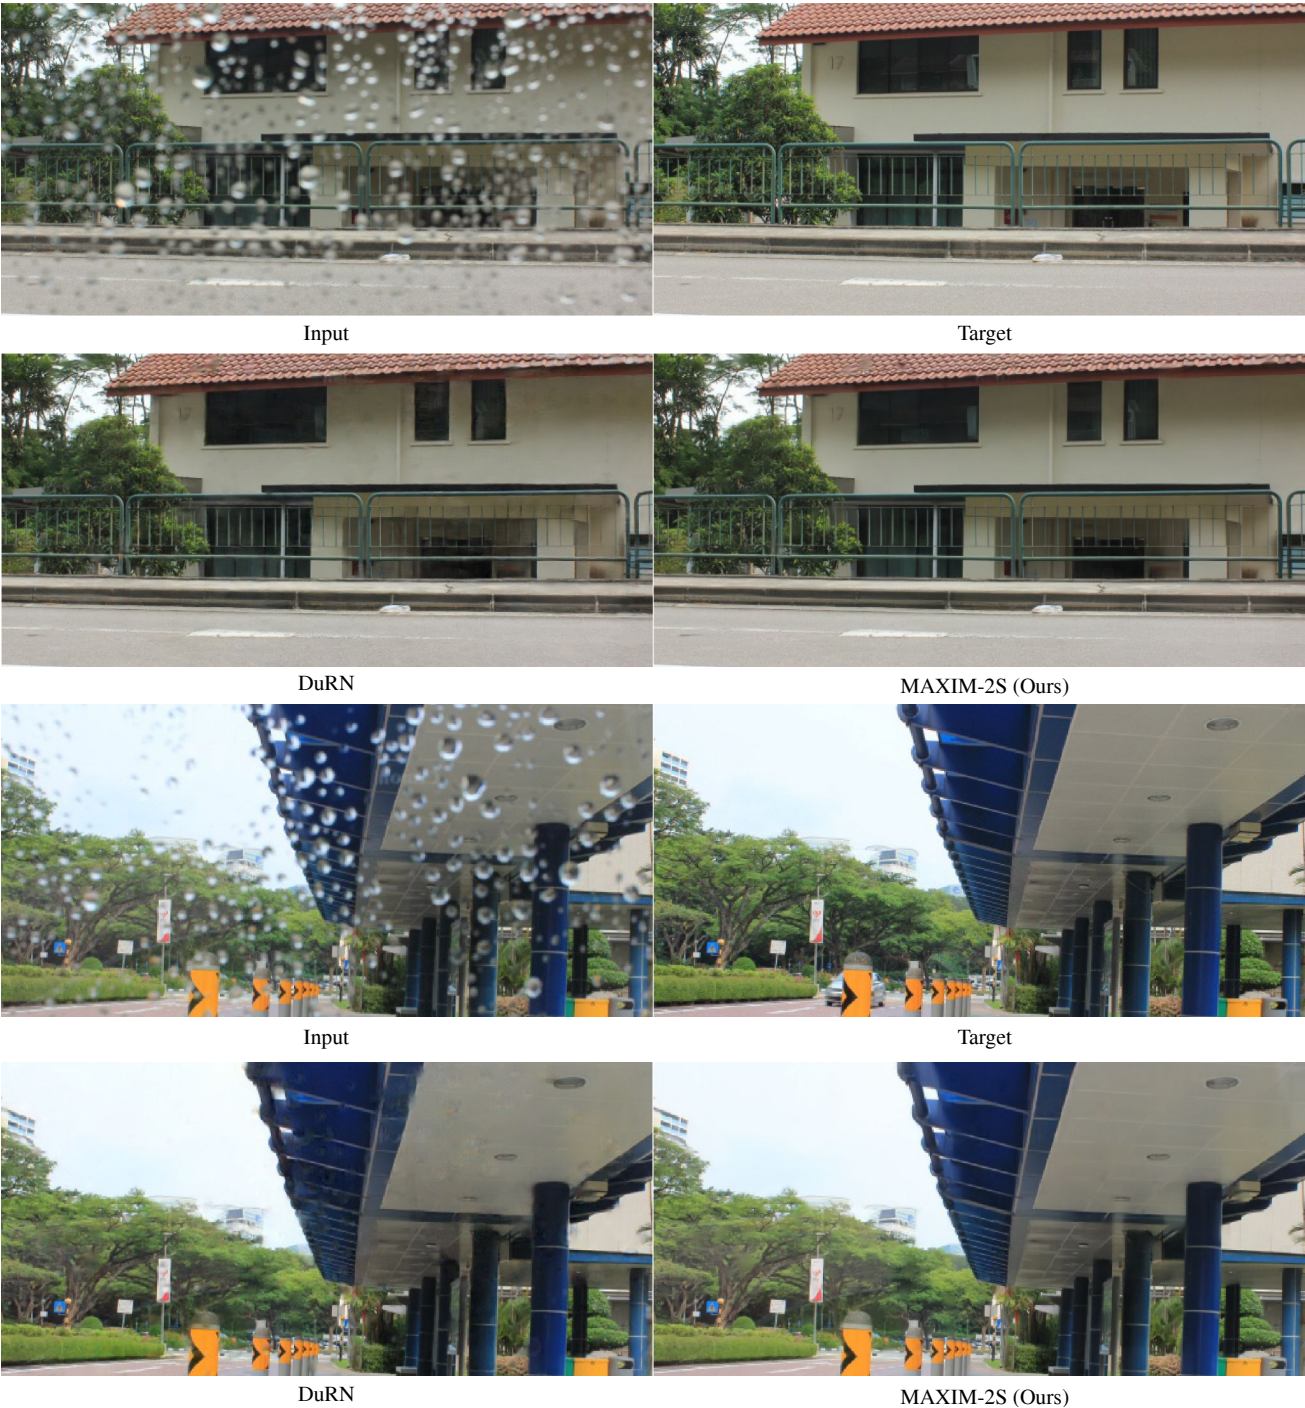

Figure 14. Visual comparisons for raindrop removal on Raindrop testset B [27].



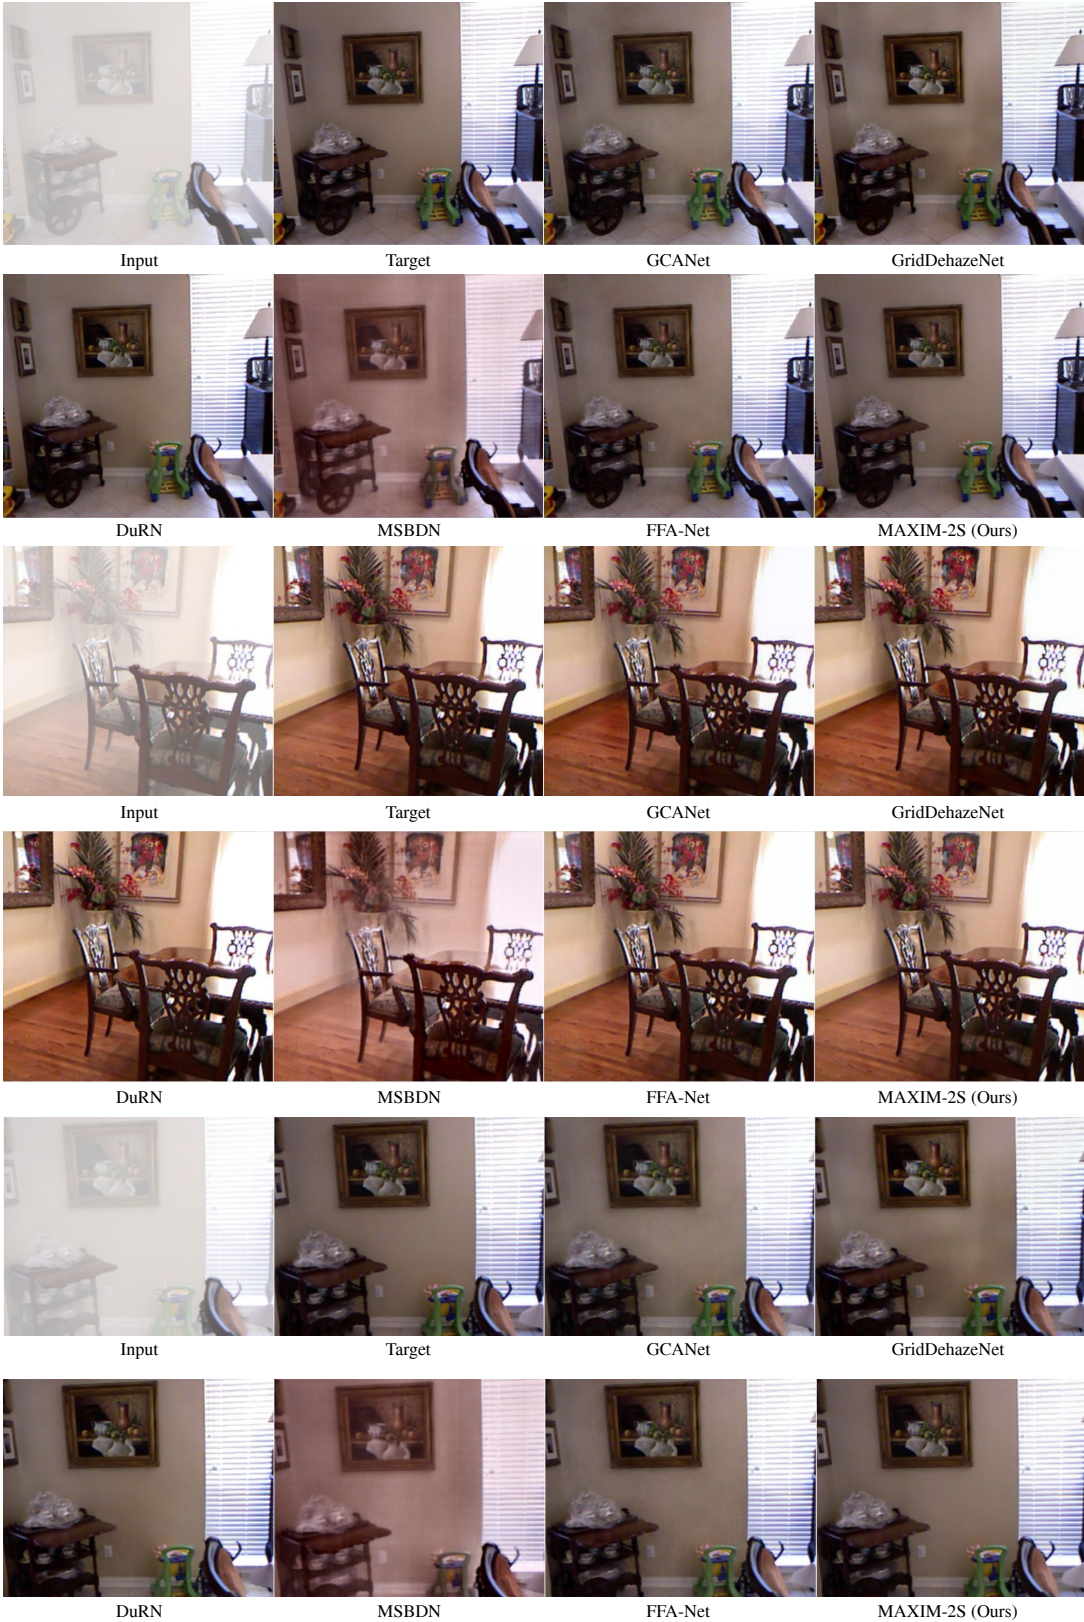

Figure 15. Visual comparisons for image dehazing on SOTS indoor testset [15] among GCANet [5], GridDehaze [19], DuRN [20], MSBDN [10], FFA-Net [28], and our MAXIM-2S.



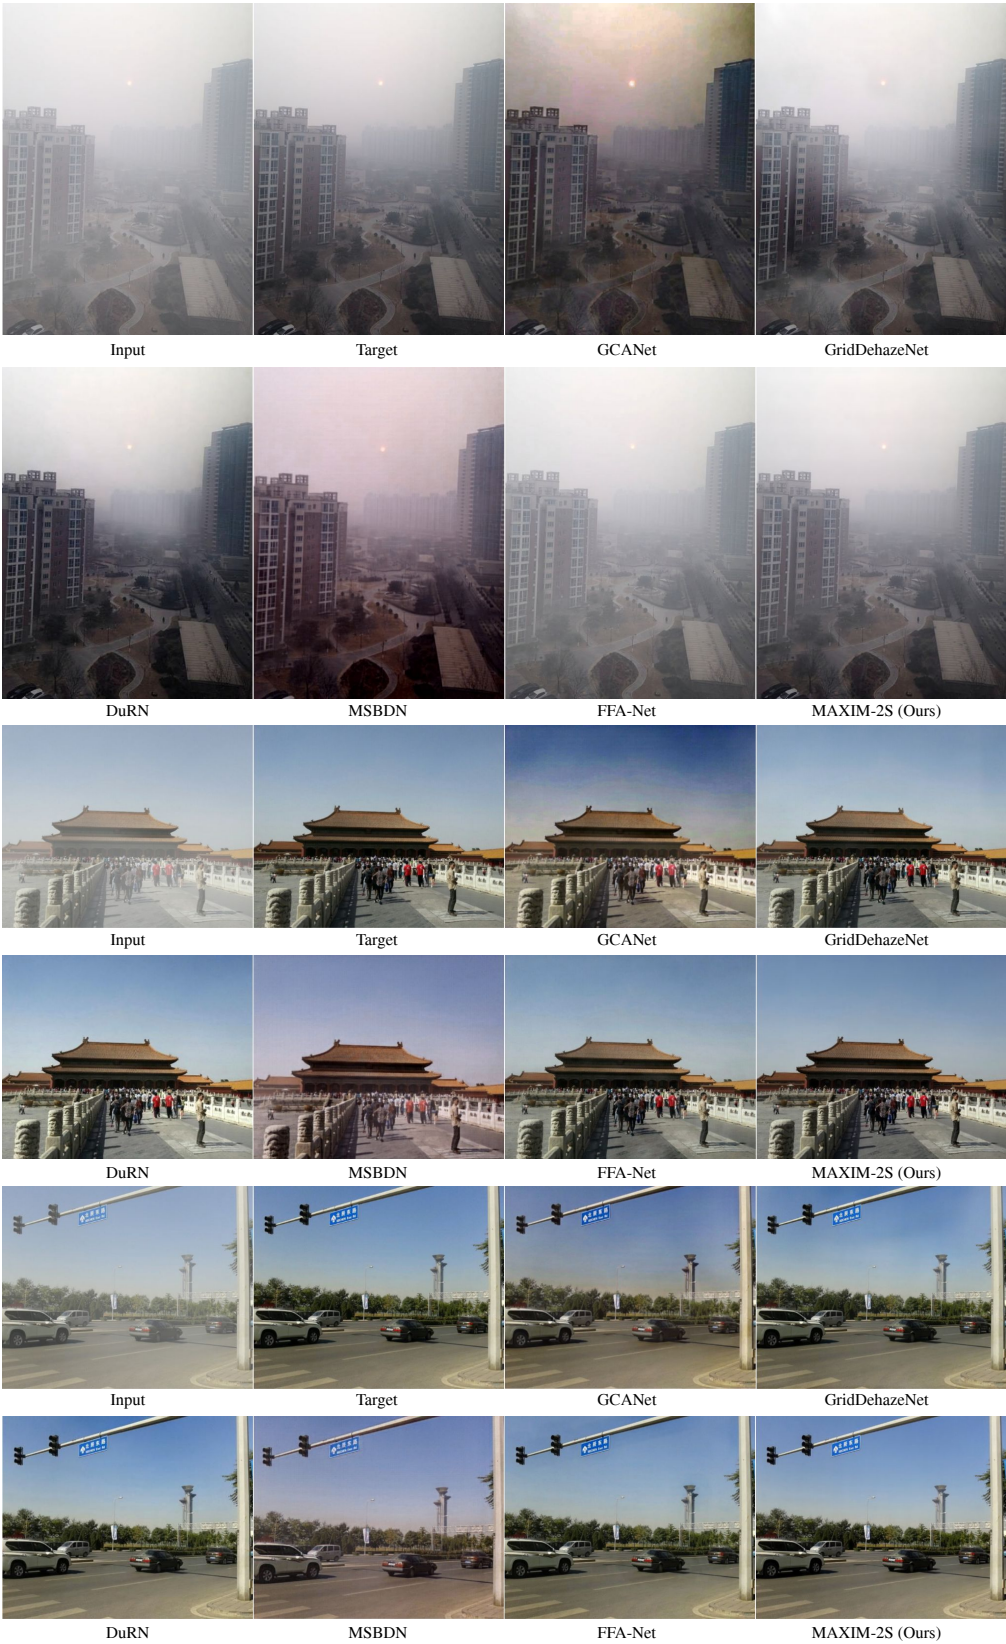

Figure 16. Visual comparisons for image dehazing on SOTS outdoor testset [15] of MAXIM-2S against other approaches.



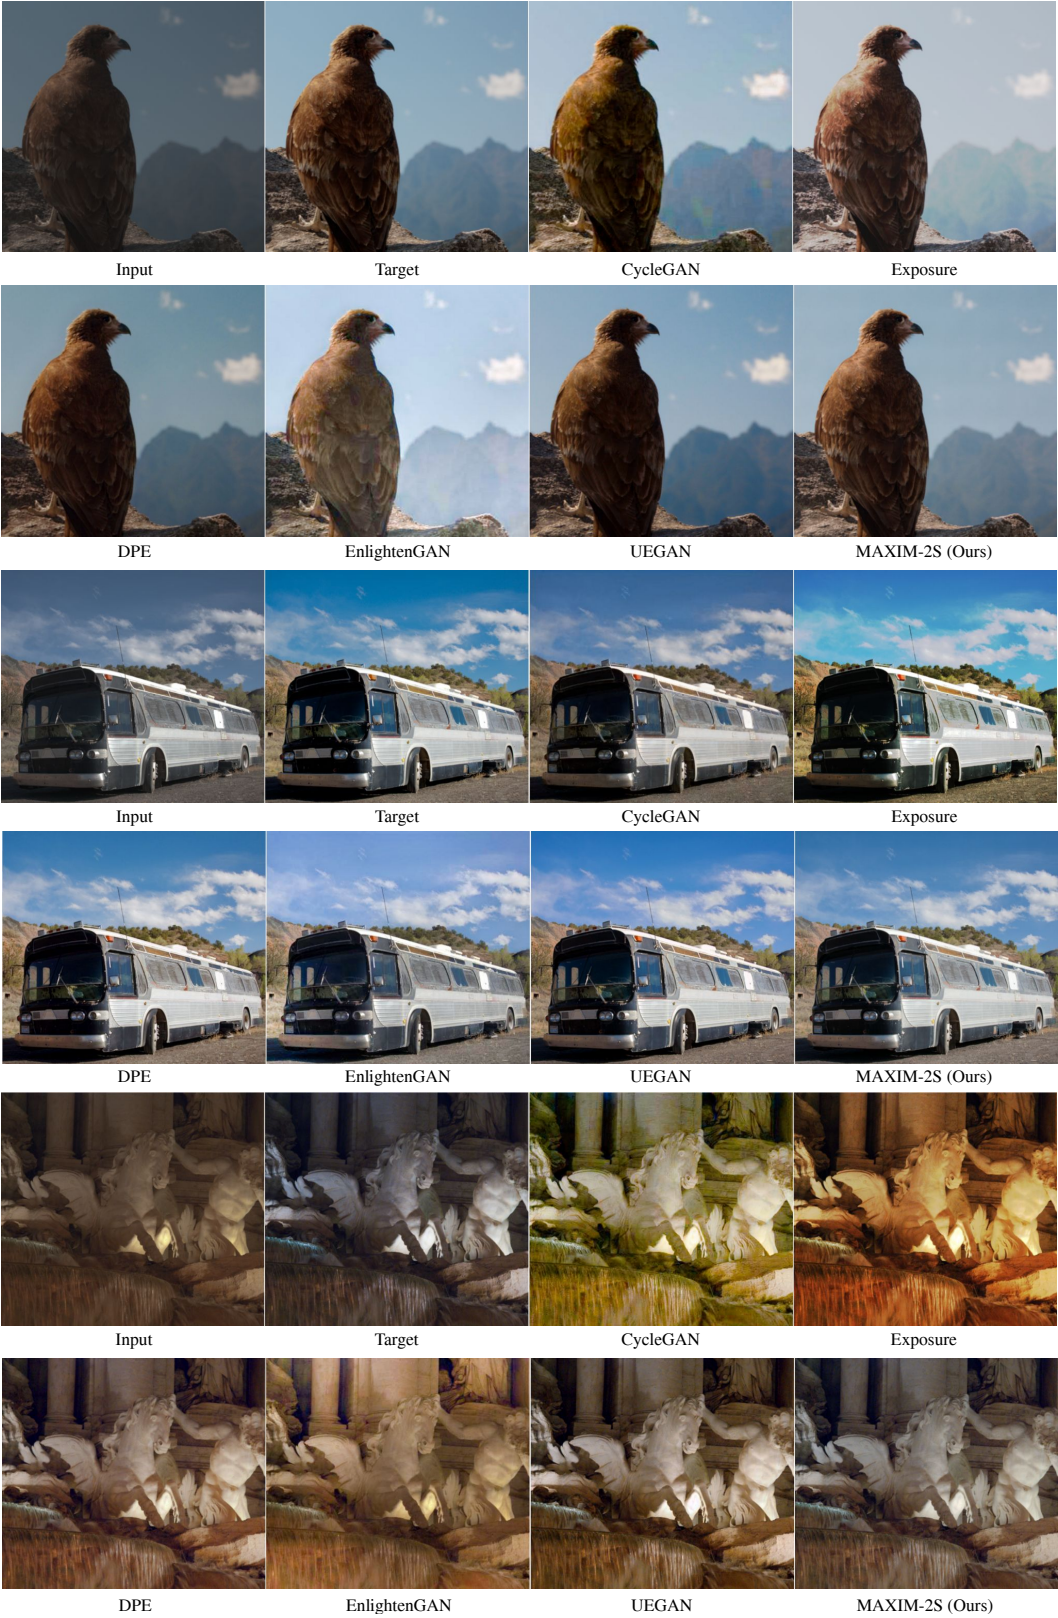

Figure 17. Visual comparisons for image retouching on MIT-Adobe FiveK [4] provided by the authors of [25] between CycleGAN [50], Exposure [12], DPE [8], EnlightenGAN, UEGAN [25] and MAXIM-2S.



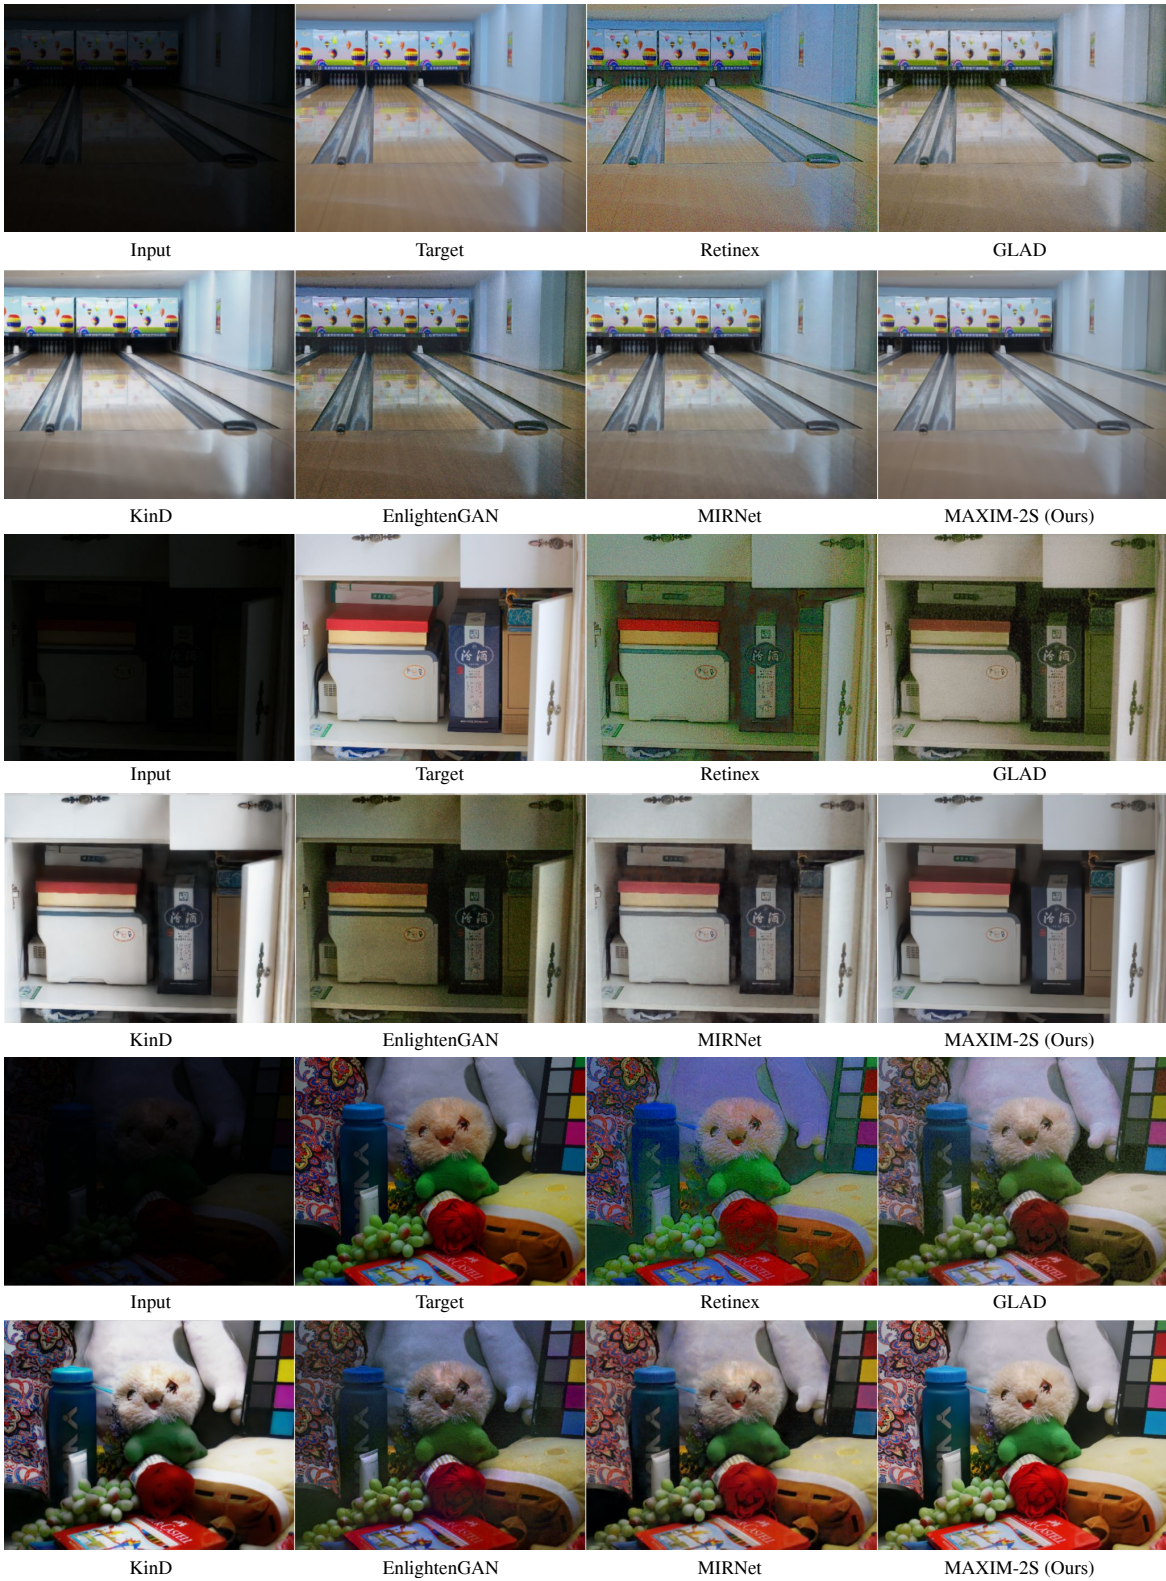

Figure 18. Visual examples for image low-light enhancement on the LOL dataset [38] between Retinex [38], GLAD [36], KinD [48], EnlightenGAN, MIRNet [43], and MAXIM-2S. Our model effectively enhances lighting while largely reducing noise, producing higher-quality images compared to other approaches.



**Algorithm 1** JAX code implementing the Multi-Axis Gated MLP Block (MAB).

---

```

from typing import Sequence
import einops
import flax.linen as nn
import jax.numpy as jnp

def block_images(x, patch_size):
    n, h, w, channels = x.shape
    grid_height, grid_width = h // patch_size[0], w // patch_size[1]
    x = einops.rearrange(x, "n_ (gh_fw) _c_ ->_n_ (gh_gw) _ (fh_fw) _c",
        gh=grid_height, gw=grid_width, fh=patch_size[0], fw=patch_size[1])
    return x

def unblock_images(x, grid_size, patch_size):
    x = einops.rearrange(x, "n_ (gh_gw) _ (fh_fw) _c_ ->_n_ (gh_fh) _ (gw_fw) _c",
        gh=grid_size[0], gw=grid_size[1], fh=patch_size[0], fw=patch_size[1])
    return x

class SpatialGatingUnit(nn.Module):
    """Gated MLP applied on a specified axis: -3 for grid and -2 for block."""
    @nn.compact
    def __call__(self, x, axis=-3):
        u, v = jnp.split(x, 2, axis=-1)
        v = nn.LayerNorm()(v)
        n = x.shape[axis] # get spatial dim at the 'grid' or 'block' axis
        v = jnp.swapaxes(v, -1, axis)
        v = nn.Dense(n)(v)
        v = jnp.swapaxes(v, -1, axis)
        return u * (v + 1.)

class SpatialGmlpLayer(nn.Module):
    """Gated MLP applied on a specified axis: -3 for grid and -2 for block."""
    grid_size: Sequence[int]
    block_size: Sequence[int]
    @nn.compact
    def __call__(self, x, axis=-3):
        n, h, w, num_channels = x.shape
        if axis=-3: # for grid gMLP layer
            gh, gw = self.grid_size
            fh, fw = h // gh, w // gw
        elif axis=-2: # for block gMLP layer
            fh, fw = self.block_size
            gh, gw = h // fh, w // fw
        x = block_images(x, patch_size=(fh, fw))
        y = nn.LayerNorm()(x)
        y = nn.Dense(num_channels * 2)(y)
        y = nn.gelu(y)
        y = SpatialGatingUnit()(y, axis=axis)
        y = nn.Dense(num_channels)(y)
        x = x + y
        x = unblock_images(x, grid_size=(gh, gw), patch_size=(fh, fw))
        return x

class MultiAxisGmlpBlock(nn.Module):
    block_size: Sequence[int]
    grid_size: Sequence[int]
    @nn.compact
    def __call__(self, x):
        shortcut = x
        n, h, w, num_channels = x.shape
        x = nn.LayerNorm()(x)
        x = nn.Dense(num_channels * 2)(x)
        x = nn.gelu(x)
        # split two heads, then applied grid gMLP and block gMLP respectively.
        u, v = jnp.split(x, 2, axis=-1)
        u = SpatialGmlpLayer(grid_size=self.grid_size)(u, axis=-3)
        v = SpatialGmlpLayer(block_size=self.block_size)(v, axis=-2)
        # Concat and output projection
        x = jnp.concatenate([u, v], axis=-1)
        x = nn.Dense(num_channels)(x)
        x = x + shortcut
        return x

```

---

## References

- [1] Darmstadt noise dataset. <https://noise.visinf.tu-darmstadt.de/benchmark>, 2017. Accessed: 2021-10-30. 1
- [2] Abdelrahman Abdelhamed, Stephen Lin, and Michael S Brown. A high-quality denoising dataset for smartphone cameras. In *CVPR*, pages 1692–1700, 2018. 1, 3, 4, 6
- [3] James Bradbury, Roy Frostig, Peter Hawkins, Matthew James Johnson, Chris Leary, Dougal Maclaurin, George Necula, Adam Paszke, Jake VanderPlas, Skye Wanderman-Milne, and Qiao Zhang. JAX: composable transformations of Python+NumPy programs, 2018. 3
- [4] Vladimir Bychkovsky, Sylvain Paris, Eric Chan, and Frédo Durand. Learning photographic global tonal adjustment with a database of input/output image pairs. In *CVPR*, pages 97–104. IEEE, 2011. 1, 2, 4, 19
- [5] Dongdong Chen, Mingming He, Qingnan Fan, Jing Liao, Liheng Zhang, Dongdong Hou, Lu Yuan, and Gang Hua. Gated context aggregation network for image dehazing and deraining. In *2019 IEEE winter conference on applications of computer vision (WACV)*, pages 1375–1383. IEEE, 2019. 17
- [6] Hanting Chen, Yunhe Wang, Tianyu Guo, Chang Xu, Yiping Deng, Zhenhua Liu, Siwei Ma, Chunjing Xu, Chao Xu, and Wen Gao. Pre-trained image processing transformer. In *CVPR*, pages 12299–12310, 2021. 3
- [7] Liangyu Chen, Xin Lu, Jie Zhang, Xiaojie Chu, and Chengpeng Chen. Hinet: Half instance normalization network for image restoration. In *CVPRW*, pages 182–192, 2021. 2, 3, 4, 7, 8, 11
- [8] Yu-Sheng Chen, Yu-Ching Wang, Man-Hsin Kao, and Yung-Yu Chuang. Deep photo enhancer: Unpaired learning for image enhancement from photographs with gans. In *CVPR*, pages 6306–6314, 2018. 19
- [9] Sung-Jin Cho, Seo-Won Ji, Jun-Pyo Hong, Seung-Won Jung, and Sung-Jea Ko. Rethinking coarse-to-fine approach in single image deblurring. In *ICCV*, pages 4641–4650, 2021. 2, 7, 8
- [10] Hang Dong, Jinshan Pan, Lei Xiang, Zhe Hu, Xinyi Zhang, Fei Wang, and Ming-Hsuan Yang. Multi-scale boosted dehazing network with dense feature fusion. In *CVPR*, pages 2157–2167, 2020. 3, 17
- [11] Xueyang Fu, Jiabin Huang, Delu Zeng, Yue Huang, Xinghao Ding, and John Paisley. Removing rain from single images via a deep detail network. In *CVPR*, pages 3855–3863, 2017. 1
- [12] Yuanming Hu, Hao He, Chenxi Xu, Baoyuan Wang, and Stephen Lin. Exposure: A white-box photo post-processing framework. *ACM TOG*, 37(2):1–17, 2018. 19
- [13] Kui Jiang, Zhongyuan Wang, Peng Yi, Chen Chen, Baojin Huang, Yimin Luo, Jiayi Ma, and Junjun Jiang. Multi-scale progressive fusion network for single image deraining. In *CVPR*, pages 8346–8355, 2020. 1, 3, 11
- [14] Yifan Jiang, Shiyu Chang, and Zhangyang Wang. Transgan: Two transformers can make one strong gan. *arXiv preprint arXiv:2102.07074*, 1(3), 2021. 4
- [15] Boyi Li, Wenqi Ren, Dengpan Fu, Dacheng Tao, Dan Feng, Wenjun Zeng, and Zhangyang Wang. Benchmarking single-image dehazing and beyond. *IEEE TIP*, 28(1):492–505, 2019. 1, 3, 4, 17, 18
- [16] Xia Li, Jianlong Wu, Zhouchen Lin, Hong Liu, and Hongbin Zha. Recurrent squeeze-and-excitation context aggregation net for single image deraining. In *ECCV*, pages 254–269, 2018. 11
- [17] Yu Li, Robby T Tan, Xiaojie Guo, Jiangbo Lu, and Michael S Brown. Rain streak removal using layer priors. In *CVPR*, pages 2736–2744, 2016. 1
- [18] Hanxiao Liu, Zihang Dai, David R So, and Quoc V Le. Pay attention to mlps. *arXiv preprint arXiv:2105.08050*, 2021. 3, 4
- [19] Xiaohong Liu, Yongrui Ma, Zhihao Shi, and Jun Chen. Grid-dehazenet: Attention-based multi-scale network for image dehazing. In *ICCV*, pages 7314–7323, 2019. 17
- [20] Xing Liu, Masanori Suganuma, Zhun Sun, and Takayuki Okatani. Dual residual networks leveraging the potential of paired operations for image restoration. In *CVPR*, pages 7007–7016, 2019. 3, 15, 17
- [21] Ze Liu, Yutong Lin, Yue Cao, Han Hu, Yixuan Wei, Zheng Zhang, Stephen Lin, and Baining Guo. Swin transformer: Hierarchical vision transformer using shifted windows. *ICCV*, 2021. 3
- [22] Seungjun Nah, Tae Hyun Kim, and Kyoung Mu Lee. Deep multi-scale convolutional neural network for dynamic scene deblurring. In *CVPR*, pages 3883–3891, 2017. 1, 3, 4, 5, 7
- [23] Seungjun Nah, Sanghyun Son, Suyoung Lee, Radu Timofte, and Kyoung Mu Lee. Ntire 2021 challenge on image deblurring. In *CVPR Workshops*, pages 149–165, June 2021. 1, 3, 4, 10
- [24] Seungjun Nah, Sanghyun Son, Suyoung Lee, Radu Timofte, and Kyoung Mu Lee. Ntire 2021 challenge on image deblurring. In *Proceedings of the IEEE/CVF Conference on Computer Vision and Pattern Recognition*, pages 149–165, 2021. 1
- [25] Zhangkai Ni, Wenhan Yang, Shiqi Wang, Lin Ma, and Sam Kwong. Towards unsupervised deep image enhancement with generative adversarial network. *IEEE TIP*, 29:9140–9151, 2020. 2, 4, 19
- [26] Tobias Plotz and Stefan Roth. Benchmarking denoising algorithms with real photographs. In *CVPR*, pages 1586–1595, 2017. 1
- [27] Rui Qian, Robby T Tan, Wenhan Yang, Jiajun Su, and Jiaying Liu. Attentive generative adversarial network for rain-drop removal from a single image. In *CVPR*, pages 2482–2491, 2018. 1, 3, 4, 15, 16
- [28] Xu Qin, Zhilin Wang, Yuanchao Bai, Xiaodong Xie, and Huizhu Jia. Ffa-net: Feature fusion attention network for single image dehazing. In *AAAI*, volume 34, pages 11908–11915, 2020. 3, 17
- [29] Yuhui Quan, Shijie Deng, Yixin Chen, and Hui Ji. Deep learning for seeing through window with raindrops. In *Proceedings of the IEEE/CVF International Conference on Computer Vision*, pages 2463–2471, 2019. 3, 15
- [30] Dongwei Ren, Wangmeng Zuo, Qinghua Hu, Pengfei Zhu, and Deyu Meng. Progressive image deraining networks: A better and simpler baseline. In *CVPR*, pages 3937–3946, 2019. 11



[31] Jaesung Rim, Haeyun Lee, Jucheol Won, and Sunghyun Cho. Real-world blur dataset for learning and benchmarking deblurring algorithms. In *ECCV*, pages 184–201. Springer, 2020. 1, 4, 9

[32] Ziyi Shen, Wenguan Wang, Xiankai Lu, Jianbing Shen, Haibin Ling, Tingfa Xu, and Ling Shao. Human-aware motion deblurring. In *ICCV*, pages 5572–5581, 2019. 1, 4, 8

[33] Sanghyun Son, Jaeha Kim, Wei-Sheng Lai, Ming-Hsuan Yang, and Kyoung Mu Lee. Toward real-world super-resolution via adaptive downsampling models. *IEEE transactions on pattern analysis and machine intelligence*, 2021. 4

[34] Maitreya Suin, Kuldeep Purohit, and AN Rajagopalan. Spatially-attentive patch-hierarchical network for adaptive motion deblurring. In *CVPR*, pages 3606–3615, 2020. 7, 8

[35] Ilya Tolstikhin, Neil Houlsby, Alexander Kolesnikov, Lucas Beyer, Xiaohua Zhai, Thomas Unterthiner, Jessica Yung, Andreas Steiner, Daniel Keysers, Jakob Uszkoreit, et al. Mlp-mixer: An all-mlp architecture for vision. *arXiv preprint arXiv:2105.01601*, 2021. 3

[36] Wenjing Wang, Chen Wei, Wenhan Yang, and Jiaying Liu. Gladnet: Low-light enhancement network with global awareness. In *2018 13th IEEE International Conference on Automatic Face & Gesture Recognition (FG 2018)*, pages 751–755. IEEE, 2018. 20

[37] Xintao Wang, Liangbin Xie, Chao Dong, and Ying Shan. Real-esrgan: Training real-world blind super-resolution with pure synthetic data. In *Proceedings of the IEEE/CVF International Conference on Computer Vision*, pages 1905–1914, 2021. 4

[38] Chen Wei, Wenjing Wang, Wenhan Yang, and Jiaying Liu. Deep retinex decomposition for low-light enhancement. *arXiv preprint arXiv:1808.04560*, 2018. 1, 2, 3, 4, 20

[39] Wenhan Yang, Robby T Tan, Jiashi Feng, Jiaying Liu, Zongming Guo, and Shuicheng Yan. Deep joint rain detection and removal from a single image. In *CVPR*, pages 1357–1366, 2017. 1, 11, 12

[40] Zongsheng Yue, Hongwei Yong, Qian Zhao, Lei Zhang, and Deyu Meng. Variational denoising network: Toward blind noise modeling and removal. *arXiv preprint arXiv:1908.11314*, 2019. 6

[41] Zongsheng Yue, Qian Zhao, Lei Zhang, and Deyu Meng. Dual adversarial network: Toward real-world noise removal and noise generation. In *ECCV*, pages 41–58. Springer, 2020. 6

[42] Syed Waqas Zamir, Aditya Arora, Salman Khan, Munawar Hayat, Fahad Shahbaz Khan, Ming-Hsuan Yang, and Ling Shao. Cycleisp: Real image restoration via improved data synthesis. In *CVPR*, pages 2696–2705, 2020. 6

[43] Syed Waqas Zamir, Aditya Arora, Salman Khan, Munawar Hayat, Fahad Shahbaz Khan, Ming-Hsuan Yang, and Ling Shao. Learning enriched features for real image restoration and enhancement. In *ECCV*, pages 492–511. Springer, 2020. 3, 6, 20

[44] Syed Waqas Zamir, Aditya Arora, Salman Khan, Munawar Hayat, Fahad Shahbaz Khan, Ming-Hsuan Yang, and Ling Shao. Multi-stage progressive image restoration. In *CVPR*, pages 14821–14831, 2021. 1, 2, 3, 4, 6, 7, 8, 9, 11

[45] Hongguang Zhang, Yuchao Dai, Hongdong Li, and Piotr Koniusz. Deep stacked hierarchical multi-patch network for image deblurring. In *CVPR*, pages 5978–5986, 2019. 7, 8

[46] He Zhang and Vishal M Patel. Density-aware single image de-raining using a multi-stream dense network. In *CVPR*, pages 695–704, 2018. 1, 14

[47] He Zhang, Vishwanath Sindagi, and Vishal M Patel. Image de-raining using a conditional generative adversarial network. *IEEE TCSVT*, 30(11):3943–3956, 2019. 1, 13

[48] Yonghua Zhang, Jiawan Zhang, and Xiaojie Guo. Kindling the darkness: A practical low-light image enhancer. In *ACM MM*, pages 1632–1640, 2019. 20

[49] Long Zhao, Zizhao Zhang, Ting Chen, Dimitris N Metaxas, and Han Zhang. Improved transformer for high-resolution gans. *arXiv preprint arXiv:2106.07631*, 2021. 4

[50] Jun-Yan Zhu, Taesung Park, Phillip Isola, and Alexei A Efros. Unpaired image-to-image translation using cycle-consistent adversarial networks. In *ICCV*, pages 2223–2232, 2017. 19
